# Supplementary material for: Nonlocal form factor of chromomagnetic penguin in $B\to K\ell^+\ell^-$ from QCD light-cone sum rules
Source: arXiv:2512.10868 ancillary file (2025-12-11)
Supplement: Supplementary file 1 [file coefficients.pdf]

# 1 Coefficients

## 1.1 Diagram in Fig 1A

This section provides the explicit coefficient functions  $\tilde{B}_i^{(j,\phi/\Phi)}$ ,  $\tilde{C}_i^{(j,\phi/\Phi)}$ , and  $\tilde{A}_i^{(j,\phi/\Phi)}$  that enter the invariant amplitudes the invariant amplitudes  $I^{(A1)}$ ,  $I^{(A2)}$ , and  $I^{(A3)}$ , respectively. The  $\phi(\Phi)$  denote the terms multiplying, respectively, the twist-2(3)  $B$ -meson distribution amplitudes. All coefficients depend on the external and kinematic variables as  $\tilde{X}_i^{(j,\phi/\Phi)} = \tilde{X}_i^{(j,\phi/\Phi)}(s, q^2, m_B, m_b, \hat{\omega}; x \text{ or } x_2, x_3)$ ,  $\hat{m}_b = \frac{m_b}{m_B}$ ,  $\hat{\omega} = \frac{\omega}{m_B}$ . A prime on  $\tilde{X}$  indicates a derivative with respect to the dispersion variable  $s$ .

•  $\tilde{B}_i^{(j,\phi/\Phi)}$ :

The coefficients used in the  $I^{(A1)}$  function ( $\tilde{B}$ ) are given below:

$$\begin{aligned} \tilde{B}_0^{(0,\phi)} = & 4 m_B (2\hat{m}_b - 1) (x - 1) x (\hat{\omega} - 1) [(\hat{\omega} - 1)(2\hat{\omega} - 5) s + ((3 - 2\hat{\omega})\hat{\omega} + 2) q^2 \\ & + m_B^2 (\hat{\omega}^2 + \hat{\omega} - 2)] , \end{aligned}$$

$$\tilde{B}_1^{(0,\phi)} = 12 m_B (2\hat{m}_b - 1) (\hat{\omega} - 1) ,$$

$$\begin{aligned} \tilde{B}_0^{(1,\Phi)} = & - 8 (x - 1) x [(\hat{\omega} - 1) s (2\hat{m}_b(\hat{\omega} - 4) - 2\hat{\omega} + 5) + q^2 (-2\hat{m}_b(\hat{\omega} - 2)\hat{\omega} + 4\hat{m}_b \\ & - 3) + m_B^2 (\hat{\omega} - 1) (4\hat{m}_b\hat{\omega} + 2\hat{m}_b - \hat{\omega} - 2)] , \end{aligned}$$

$$\tilde{B}_1^{(1,\Phi)} = - 24 (2\hat{m}_b - 1) ,$$

$$\begin{aligned} \tilde{B}_0^{(2,\Phi)} = & - 8 x [ - (2\hat{m}_b + 1)(\hat{\omega} - 1) s + q^2 (2\hat{m}_b(\hat{\omega} - 2) - 3\hat{\omega} + 4) + m_B^2 (\hat{\omega} - 1) \\ & (6\hat{m}_b\hat{\omega} - 4\hat{m}_b - 3\hat{\omega} + 4)] , \end{aligned}$$

$$\tilde{B}_1^{(2,\Phi)} = 0 ,$$

$$\begin{aligned} \tilde{B}_0^{(3,\Phi)} = & - 8 (x - 1) x \left\{ - (\hat{\omega} - 1) q^2 [s (2\hat{m}_b(\hat{\omega} - 4) - 5\hat{\omega} + 11) + m_B^2 (2\hat{m}_b(2(\hat{\omega} - 2)\hat{\omega}^2 + \hat{\omega} + 4) \right. \\ & + \hat{\omega}((7 - 2\hat{\omega})\hat{\omega} - 3) - 8)] + (\hat{\omega} - 1)^2 s [(5 - 2\hat{\omega}) s + 2m_B^2 (\hat{m}_b(\hat{\omega} - 1)(2\hat{\omega} - 5) \\ & - (\hat{\omega} - 4)\hat{\omega} - 6)] + q^4 (2\hat{m}_b((\hat{\omega} - 2)\hat{\omega} - 2) + \hat{\omega}(2(\hat{\omega} - 3)\hat{\omega} + 3) + 4) \\ & \left. + m_B^4 (\hat{\omega} - 1)^2 (\hat{\omega} + 2) (2\hat{m}_b(\hat{\omega} - 1) - \hat{\omega} + 2) \right\} , \end{aligned}$$

$$\tilde{B}_1^{(3,\Phi)} = - 24 (- q^2 (2\hat{m}_b + \hat{\omega} - 2) - (\hat{\omega} - 1) s + m_B^2 (\hat{\omega} - 1) (2\hat{m}_b(\hat{\omega} - 1) - \hat{\omega} + 2)) ,$$

$$\tilde{B}_0^{(4,\Phi)} = 8 (x - 1)^2 x \left\{ - (\hat{\omega} - 2)(\hat{\omega} - 1) q^2 [s (-2\hat{m}_b(\hat{\omega} - 4) + 5\hat{\omega} - 11) \right.$$

$$\begin{aligned}
& + m_B^2 \left( 2\hat{m}_b((\hat{\omega} - 1)\hat{\omega} - 3) + (3 - 4\hat{\omega})\hat{\omega} + 7 \right) ] + (\hat{\omega} - 1)^2 s [(\hat{\omega} - 2)(2\hat{\omega} - 5) s \\
& + m_B^2 (2\hat{m}_b(\hat{\omega} - 1)(2\hat{\omega} - 5) + (16 - 3\hat{\omega})\hat{\omega} - 19) ] - (\hat{\omega} - 2) q^4 (2\hat{m}_b((\hat{\omega} - 2)\hat{\omega} - 2) \\
& + \hat{\omega}(2(\hat{\omega} - 3)\hat{\omega} + 3) + 4) + m_B^4 (\hat{\omega} - 1)^2 (\hat{\omega} + 2) (2\hat{m}_b(\hat{\omega} - 1) - 2\hat{\omega} + 3) \Big\} ,
\end{aligned}$$

$$\begin{aligned}
\tilde{B}_1^{(4,\Phi)} = & 4 \Big( - (\hat{\omega} - 1) s (\hat{\omega} (3\hat{m}_b(x - 1) - 5x + 7) + 4\hat{m}_b + 14x - 15) \\
& + q^2 (\hat{\omega}^2 (3\hat{m}_b(x - 1) + 5x - 3) + \hat{\omega} (\hat{m}_b(11x - 7) - 21x + 18) - 26\hat{m}_b x + 24\hat{m}_b \\
& + 25x - 23) + m_B^2 (\hat{\omega} - 1) (\hat{m}_b (3x(7\hat{\omega} - 6) - 15\hat{\omega} + 16) - 14x\hat{\omega} + 23x + 13\hat{\omega} - 21) \\
& - 2(\hat{m}_b (\hat{\omega} (2(x - 1)\hat{\omega} + x + 3) - 2) + x\hat{\omega}(4\hat{\omega} - 5) + x - \hat{\omega} + 1) \Big) .
\end{aligned}$$

$$\bullet \underline{\tilde{C}_i^{(j,\phi/\Phi)}} :$$

The coefficients used in the  $I^{(A2)}$  function ( $\tilde{C}$ ) are given below with the following shorthand parameter combinations:

$$\begin{aligned}
b_1 &= -(x_2 + x_3), & b_2 &= x_2 + x_3, & b_3 &= x_3, \\
b_4 &= 1 - (x_2 + x_3), & b_5 &= x_2 + x_3 - 1, & b_6 &= x_3 - 1, \\
b_{12} &= b_1 \hat{\omega} + b_2, & b_{13} &= b_1 \hat{\omega} + b_3, & b_{45} &= b_4 \hat{\omega} + b_5, \\
b_{43} &= b_4 \hat{\omega} + b_3 & b_{46} &= b_4 \hat{\omega} + b_6.
\end{aligned}$$

$$\begin{aligned}
\tilde{C}_0^{(0,\phi)} = & -4m_B \left( s [b_{12} (b_{43}b_{45}(3 - 4\hat{\omega}) + 4b_{43}b_{46}(\hat{\omega} - 1) + b_{45}^2\hat{\omega} - 3b_{45}b_{46}(\hat{\omega} - 1)) \right. \\
& + b_{13}b_{45}(\hat{\omega} - 1)(3b_{45} - b_{46})] + q^2 [b_{43}\hat{\omega}(b_{13} - b_{12})(b_{45} - 3b_{46}) - 4b_{12}b_{43}b_{46} \\
& \left. + b_{13}b_{46}(3b_{43} + b_{45})] + m_B^2 [b_{12}b_{43}(b_{45}\hat{\omega} - 4b_{46}(\hat{\omega} - 1)) + b_{13}b_{45}b_{46}(\hat{\omega} - 1)] \right) ,
\end{aligned}$$

$$\tilde{C}_1^{(0,\phi)} = -2m_B (b_{12}\hat{\omega} + 3b_{13}(\hat{\omega} - 1) + 2\hat{\omega}(-3b_{43} + b_{45} - 3b_{46}) + 6(b_{43} + b_{46})) ,$$

$$\begin{aligned}
\tilde{C}_0^{(1,\Phi)} = & -8 \left( s [2b_{12}b_{43}(b_{45} - b_{46}) + b_{12}b_{45}(b_{45} + 3b_{46}) - b_{13}b_{45}(3b_{45} + b_{46})] + b_{43}q^2(b_{13} - b_{12}) \right. \\
& \left. (b_{45} + 3b_{46}) + m_B^2 [b_{12}b_{43}(b_{45} + 2b_{46}) + b_{13}b_{45}b_{46}] \right) ,
\end{aligned}$$

$$\tilde{C}_1^{(1,\Phi)} = -4 (b_{12} - 3b_{13} + 6b_{43} + 2b_{45} + 6b_{46}) ,$$

$$\tilde{C}_0^{(2,\Phi)} = -8 \left( (b_{12} - b_{13}) [s (b_{45}\hat{\omega} + b_{45} - b_{46}\hat{\omega} + b_{46}) + q^2 (b_{46}(\hat{\omega} - 2) - b_{45}\hat{\omega})] + m_B^2 [b_{12}b_{45}\hat{\omega} \right.$$

$$- 2b_{12}b_{46}(\hat{\omega} - 1) + b_{13}(2b_{45}\hat{\omega} + b_{46}(1 - \hat{\omega}))],$$

$$\tilde{C}_1^{(2,\Phi)} = -12,$$

$$\begin{aligned} \tilde{C}_0^{(3,\Phi)} = & 8(s[b_{12}(b_{43} + 2b_{45}\hat{\omega} - 3b_{45}) - 2b_{13}b_{45}(\hat{\omega} - 1)] - q^2[2b_{12}b_{43}(\hat{\omega} - 2) + b_{13}(-2b_{43}\hat{\omega} \\ & + 3b_{43} + b_{45})] + m_B^2[b_{12}b_{43}(3\hat{\omega} - 4) - b_{13}b_{45}(\hat{\omega} - 1)]), \end{aligned}$$

$$\tilde{C}_1^{(3,\Phi)} = 8(2\hat{\omega} - 3),$$

$$\begin{aligned} \tilde{C}_0^{(4,\Phi)} = & 8\left(s\left\{q^2(b_{45} - b_{46})[\hat{\omega}(b_{12} - b_{13})(b_{43} - b_{45})(b_{45} - b_{46}) - 3b_{12}b_{43}b_{45} + 3b_{12}b_{43}b_{46} \right. \right. \\ & - 4b_{12}b_{45}b_{46} + b_{13}b_{43}b_{45} - b_{13}b_{43}b_{46} + 2b_{13}b_{45}^2 + 2b_{13}b_{45}b_{46}] + b_{45}m_B^2[b_{12}(b_{43}b_{45}(3 - 4\hat{\omega}) \\ & + 4b_{43}b_{46}(\hat{\omega} - 1) + b_{45}^2\hat{\omega} - 4b_{45}b_{46}(\hat{\omega} - 1) + b_{46}^2(\hat{\omega} - 1)) + 2b_{13}(\hat{\omega} - 1)(b_{45}^2 + b_{45}b_{46} - b_{46}^2)]\Big\} \\ & + m_B^2q^2[-2b_{12}b_{43}(b_{45}^2\hat{\omega} + b_{45}b_{46}(4 - 3\hat{\omega}) + b_{46}^2(\hat{\omega} - 2)) + b_{13}b_{43}\hat{\omega}(b_{45}^2 - 4b_{45}b_{46} + b_{46}^2) \\ & + b_{13}b_{46}(4b_{43}b_{45} - b_{43}b_{46} + b_{45}b_{46})] + b_{43}q^4(b_{12} - b_{13})(b_{45} - b_{46})(b_{45}\hat{\omega} - b_{46}(\hat{\omega} - 4)) \\ & \left. - b_{45}(\hat{\omega} - 1)s^2(b_{12} - b_{13})(b_{45} - b_{46})^2 + b_{45}m_B^4[b_{12}b_{43}(b_{45}\hat{\omega} - 4b_{46}(\hat{\omega} - 1)) + b_{13}b_{46}^2(\hat{\omega} - 1)]\right), \end{aligned}$$

$$\begin{aligned} \tilde{C}_1^{(4,\Phi)} = & -4\left(s[b_{12}(b_{43} + b_{45}(\hat{\omega} - 5) + b_{46}(\hat{\omega} - 2)) + b_{13}(-\hat{\omega}(b_{45} + b_{46}) + 5b_{45} + b_{46}) \right. \\ & - 2\hat{\omega}(b_{45} - b_{46})(b_{43} - b_{45} + b_{46}) - 2(b_{43}(b_{45} + b_{46}) + b_{46}(b_{46} - 2b_{45}))] \\ & + q^2[b_{12}(\hat{\omega}(b_{45} - b_{46}) - 2b_{43}(\hat{\omega} - 2)) + b_{13}(b_{43}(2\hat{\omega} - 3) - b_{45}(\hat{\omega} + 2) + b_{46}\hat{\omega} + b_{46}) \\ & + 2(b_{43}(\hat{\omega} + 2)(b_{45} - b_{46}) + \hat{\omega}(b_{45} - b_{46})^2 + b_{46}(5b_{45} - 4b_{46}))] + \hat{\omega}[m_B^2(b_{12}(3b_{43} - b_{45} + b_{46}) \\ & + b_{43}(8b_{45} - 2b_{46}) - 2(b_{45}^2 - 5b_{45}b_{46} + b_{46}^2)) - 2(b_{45} - b_{46})(b_{12} + b_{43} - b_{45})] \\ & - 2(2b_{12}b_{46} + 2b_{43}(b_{45} + b_{46}) + b_{45}^2 - b_{45}b_{46}) + 2m_B^2(-2b_{43}(b_{12} + b_{45}) + b_{46}(b_{43} - 5b_{45}) + b_{46}^2) \\ & \left. + b_{13}(2b_{45}(m_B^2(1 - 3\hat{\omega}) + \hat{\omega} + 1) + b_{46}(m_B^2 - 2)(\hat{\omega} - 1))\right), \end{aligned}$$

$$\tilde{C}_2^{(4,\Phi)} = -4(2\hat{\omega} - 3),$$

$$\tilde{C}_0^{(5,\Phi)} = 8\left(s\left\{q^2[\hat{\omega}(b_{12} - b_{13})(b_{45} - b_{43})(b_{45} - b_{46}) + 3b_{12}b_{43}b_{45} - 3b_{12}b_{43}b_{46} + 4b_{12}b_{45}b_{46} - b_{13}b_{43}b_{45} \right. \right.$$

$$\begin{aligned}
& + b_{13}b_{43}b_{46} - 2b_{13}b_{45}^2 - 2b_{13}b_{45}b_{46}] - m_B^2(\hat{\omega} - 1)[b_{12}b_{43}(b_{45}(4\hat{\omega} - 3) - 4b_{46}(\hat{\omega} - 1)) \\
& - b_{12}b_{45}(b_{45}\hat{\omega} + b_{46}(4 - 3\hat{\omega})) + b_{13}b_{45}(-3b_{45}\hat{\omega} + 2b_{45} + b_{46}\hat{\omega} + b_{46})] \Big\} \\
& + m_B^2q^2[-b_{12}b_{43}b_{45}(\hat{\omega} - 2)\hat{\omega} + b_{12}b_{43}b_{46}(3(\hat{\omega} - 3)\hat{\omega} + 8) + b_{13}b_{43}(\hat{\omega} - 1)(b_{45}\hat{\omega} \\
& + b_{46}(4 - 3\hat{\omega})) + b_{13}b_{45}b_{46}\hat{\omega}] + b_{43}q^4(b_{12} - b_{13})(b_{46}(\hat{\omega} - 4) - b_{45}\hat{\omega}) + b_{45}(\hat{\omega} - 1)s^2 \\
& (b_{12} - b_{13})(b_{45} - b_{46}) + m_B^4(\hat{\omega} - 1)[b_{12}b_{43}(b_{45}\hat{\omega} - 4b_{46}(\hat{\omega} - 1)) + b_{13}b_{45}b_{46}\hat{\omega}]) \Big), \\
\tilde{C}_1^{(5,\Phi)} = & 4(q^2(\hat{\omega}(b_{12} + b_{43} + 2b_{45} - 2b_{46}) - b_{13}(\hat{\omega} + 2) + 5b_{43} + 8b_{46}) + (\hat{\omega} - 1)s(b_{12} - b_{13} + b_{43} - 2b_{46}) \\
& + (\hat{\omega} - 1)(m_B^2\hat{\omega}(b_{12} + 3b_{13} + 2b_{45} - 6b_{46}) - 2m_B^2(b_{13} - 4b_{46}) + b_{43}(m_B^2(5 - 6\hat{\omega}) + 2) + 2b_{45})) \Big), \\
\tilde{C}_2^{(5,\Phi)} = & 0, \\
\tilde{C}_0^{(6,\Phi)} = & 8\Big(s[b_{45}m_B^2(b_{12}(b_{43}b_{45}(3 - 4\hat{\omega}) + 5b_{43}b_{46}(\hat{\omega} - 1) + b_{45}^2\hat{\omega} - 4b_{45}b_{46}(\hat{\omega} - 1)) + b_{13}(\hat{\omega} - 1) \\
& (b_{43}(b_{45} - 2b_{46}) + b_{45}(2b_{45} + b_{46})))] - q^2(b_{43} - b_{45})[\hat{\omega}(b_{12} - b_{13})(b_{43} - b_{45})(b_{45} - b_{46}) \\
& - 3b_{12}b_{43}b_{45} + 3b_{12}b_{43}b_{46} - 4b_{12}b_{45}b_{46} + b_{13}b_{43}b_{45} - b_{13}b_{43}b_{46} + 2b_{13}b_{45}^2 + 2b_{13}b_{45}b_{46}] \\
& + b_{43}q^2[q^2(b_{12} - b_{13})(b_{43} - b_{45})(b_{46}(\hat{\omega} - 4) - b_{45}\hat{\omega}) + m_B^2(b_{12}b_{43}(b_{45}\hat{\omega} - 2b_{46}(\hat{\omega} - 2)) \\
& + b_{12}b_{45}(b_{46}(5\hat{\omega} - 8) - 2b_{45}\hat{\omega}) + b_{13}b_{43}b_{46}(\hat{\omega} - 1) + b_{13}b_{45}(b_{45}\hat{\omega} + b_{46}(5 - 4\hat{\omega})))]) \\
& + b_{45}(\hat{\omega} - 1)s^2(b_{12} - b_{13})(b_{43} - b_{45})(b_{45} - b_{46}) + b_{43}b_{45}m_B^4(b_{12}b_{45}\hat{\omega} - 4b_{12}b_{46}(\hat{\omega} - 1) \\
& + b_{13}b_{46}(\hat{\omega} - 1)) \Big), \\
\tilde{C}_1^{(6,\Phi)} = & 4\Big(s[b_{12}(b_{43}(\hat{\omega} - 2) - \hat{\omega}(b_{45} + 2b_{46}) + 5b_{45} + 3b_{46}) + b_{13}(-\hat{\omega}b_{43} + b_{43} + b_{45}(\hat{\omega} - 5) \\
& + 2b_{46}(\hat{\omega} - 1)) + \hat{\omega}(b_{43}^2 + 2b_{43}b_{45} - 5b_{43}b_{46} - 2b_{45}^2 + 4b_{45}b_{46}) - b_{43}^2 + 2b_{43}b_{45} + 5b_{43}b_{46} \\
& - 4b_{45}b_{46}] + q^2[b_{12}(b_{43}(3\hat{\omega} - 4) - b_{45}\hat{\omega}) + b_{13}(-3b_{43}\hat{\omega} + b_{43} + b_{45}(\hat{\omega} + 2) + b_{46}) \\
& + \hat{\omega}(b_{43}^2 - b_{43}b_{46} + 2b_{45}(b_{46} - b_{45})) + 5b_{43}^2 - 4b_{43}b_{45} + 7b_{43}b_{46} - 10b_{45}b_{46}] \\
& + b_{43}[m_B^2(b_{12}(4 - 3\hat{\omega}) + b_{13}(\hat{\omega} - 1)) + b_{45}(m_B^2(4 - 8\hat{\omega}) + 4\hat{\omega} + 2) + b_{46}(5m_B^2(\hat{\omega} - 1) \\
& - 4\hat{\omega} + 6)] + \hat{\omega}[b_{12}(m_B^2 + 2)(b_{45} - b_{46}) + 2m_B^2(b_{45}(3b_{13} + b_{45}) - b_{46}(b_{13} + 5b_{45}))]
\end{aligned}$$

$$\begin{aligned}
& -2b_{45}(b_{13} + b_{45}) + 2b_{13}b_{46}] + 4b_{12}b_{46} - 2b_{13}(m_B^2(b_{45} - b_{46}) + b_{45} + b_{46}) \\
& - (b_{43}^2(m_B^2 - 2)(\hat{\omega} - 1)) + 2b_{45}(b_{45} + 5b_{46}m_B^2) \Big), \\
\end{aligned}$$

$$\tilde{C}_2^{(6,\Phi)} = -4(2\hat{\omega} - 3).$$

•  $\tilde{A}_i^{(j,\phi/\Phi)}$ :

The coefficients used in the  $I^{(A3)}$  function ( $\tilde{A}$ ) are given below:

$$\begin{aligned}
\tilde{A}_0^{(0,\phi)} &= 12b_{1t}^2 m_B^3 (\hat{\omega} - 1)(2\hat{\omega} - 1), & \tilde{A}_1^{(0,\phi)} &= 12m_B (\hat{\omega} - 1)(2\hat{\omega} - 1), \\
\tilde{A}_0^{(1,\Phi)} &= \tilde{A}_1^{(1,\Phi)} = \tilde{A}_1^{(3,\Phi)} = 0, & \tilde{A}_0^{(2,\Phi)} &= -24b_{1t}^2 m_B^2 (2\hat{\omega} - 1), \\
\tilde{A}_1^{(2,\Phi)} &= -24(2\hat{\omega} - 1), & \tilde{A}_0^{(3,\Phi)} &= -16b_{1t} m_B^2 (\hat{\omega} - 1), \\
\tilde{A}_0^{(4,\Phi)} &= -24b_{1t}^2 m_B^4 (\hat{\omega} - 1)(2(\hat{\omega} - 1)\hat{\omega} + 1), \\
\tilde{A}_1^{(4,\Phi)} &= -24m_B^2 (\hat{\omega} - 1)(2(\hat{\omega} - 1)\hat{\omega} + 1), \\
\tilde{A}_0^{(5,\Phi)} &= -24b_{1t}^2 m_B^4 (\hat{\omega} - 1)^2(2\hat{\omega} - 1), & \tilde{A}_1^{(5,\phi)} &= -24m_B^2 (\hat{\omega} - 1)^2(2\hat{\omega} - 1), \\
\tilde{A}_0^{(6,\Phi)} &= -24b_{1t}^3 m_B^4 (\hat{\omega} - 1)(2\hat{\omega} - 1), & \tilde{A}_1^{(6,\phi)} &= -36b_{1t} m_B^2 (\hat{\omega} - 1)(2\hat{\omega} - 1).
\end{aligned}$$

where,

$$b_{1t} = (1 - \hat{\omega})(x - 1).$$

## 1.2 Diagram in Fig 1B

This section provides the explicit coefficient functions  $\bar{A}_i^{(j,\phi/\Phi)}$ ,  $\bar{C}_i^{(j,\phi/\Phi)}$ , and  $\bar{B}_i^{(j,\phi/\Phi)}$  that enter the invariant amplitudes the invariant amplitudes  $I^{(B1)}$ ,  $I^{(B2)}$ , and  $I^{(B3)}$ , respectively. The  $\phi(\Phi)$  denote the terms multiplying, respectively, the twist-two(three)  $B$ -meson distribution amplitudes. All coefficients depend on the external and kinematic variables as  $\bar{X}_i^{(j,\phi/\Phi)} = \bar{X}_i^{(j,\phi/\Phi)}(s, q^2, m_B, m_b, \hat{\omega}; x \text{ or } x_2, x_3)$ ,  $\hat{m}_b = \frac{m_b}{m_B}$ ,  $\hat{\omega} = \frac{\omega}{m_B}$ . A prime on  $\tilde{X}$  indicates a derivative with respect to the dispersion variable  $s$ .

•  $\bar{A}_i^{(j,\phi/\Phi)}$ :

The coefficients used in the  $I^{(B1)}$  function ( $\bar{A}$ ) are given below:

$$\begin{aligned}
\bar{A}_0^{(0,\phi)} &= 12m_B(x - 1)(\hat{m}_b + \hat{\omega} - 1)(-\hat{m}_b s + (\hat{m}_b - 1)q^2 + m_B^2\hat{m}_b), \\
\bar{A}_1^{(0,\phi)} &= 12m_B(2\hat{m}_b - 1)(1 - \hat{\omega}), \\
\bar{A}_0^{(1,\Phi)} &= 24(2\hat{m}_b - 1)(x - 1)(-\hat{m}_b s + (\hat{m}_b - 1)q^2 + m_B^2\hat{m}_b), \\
\bar{A}_1^{(1,\Phi)} &= 24(2\hat{m}_b - 1),
\end{aligned}$$

$$\bar{A}_0^{(2,\Phi)} = -24(x-1) \left( -\hat{m}_b s + (\hat{m}_b - 1)q^2 + m_B^2 \hat{m}_b \right) \left( (2\hat{m}_b + \hat{\omega} - 2)(q^2 + m_B^2(\hat{\omega} - 1)) + (\hat{\omega} - 1)s \right),$$

$$\bar{A}_1^{(2,\Phi)} = 24 \left( -q^2(2\hat{m}_b + \hat{\omega} - 2) - (\hat{\omega} - 1)s + m_B^2(\hat{\omega} - 1)(2\hat{m}_b(\hat{\omega} - 1) - \hat{\omega} + 2) \right).$$

$$\bullet \bar{C}_i^{(j,\phi/\Phi)}:$$

The coefficients used in the  $I^{(B2)}$  function ( $\bar{C}$ ) are given below with the following shorthand parameter combinations:

$$c_1 = -(x_2 + x_3), \quad c_2 = x_3, \quad c_3 = 1 - (x_2 + x_3), \quad c_4 = x_3 - 1,$$

$$c_{10} = c_1 m_b, \quad c_{12} = c_1 m_b + c_2, \quad c_{30} = c_3 m_b,$$

$$c_{32} = c_3 m_b + c_2, \quad c_{34} = c_3 m_b + c_4.$$

$$\begin{aligned} \bar{C}_0^{(0,\phi)} = & -4 \left( s \left[ c_{10} (c_{30}^2 m_B \hat{\omega} + c_{32} m_B (c_{30}(2\hat{\omega} - 3) - 2c_{34}(\hat{\omega} - 1)) - c_{34}(\hat{\omega} - 1)(2m_b - 3c_{30}m_B) \right. \right. \\ & \left. \left. - 4c_{32}m_b(\hat{\omega} - 1)) + c_{12}(\hat{\omega} - 1)(-c_{30}m_B(3c_{30} + c_{34}) + 4c_{32}m_b + 2c_{34}m_b) \right] \right. \\ & + q^2 [\hat{\omega}(c_{10} - c_{12})(-c_{32}m_B(c_{30} + 3c_{34}) + 2c_{32}m_b + 4c_{34}m_b) + 2c_{10}c_{32}c_{34}m_B \\ & + c_{10}c_{32}m_b - c_{10}c_{34}m_b + c_{12}c_{30}c_{34}m_B - 3c_{12}c_{32}c_{34}m_B - c_{12}c_{32}m_b + c_{12}c_{34}m_b] \\ & + m_B [c_{10}(c_{32}m_B(c_{30}m_B\hat{\omega} + 2c_{34}m_B(\hat{\omega} - 1) + m_b(\hat{\omega} - 1)) - m_b\hat{\omega}(c_{34}m_B + m_b) \\ & \left. \left. + c_{34}m_b m_B) + c_{12}(\hat{\omega} - 1)(c_{30}c_{34}m_B^2 - 2m_b m_B(2c_{32} + c_{34}) + 3m_b^2) \right] \right), \end{aligned}$$

$$\bar{C}_1^{(0,\phi)} = -2 \left( m_B \hat{\omega} (c_{10} - 3c_{12} + 2c_{30} + 6(c_{32} + c_{34})) + 3m_B (c_{12} - 2(c_{32} + c_{34})) + m_b(3 - 6\hat{\omega}) \right),$$

$$\begin{aligned} \bar{C}_0^{(1,\Phi)} = & -8 \left( s \left[ c_{10} (c_{30}^2 - 4c_{30}c_{32} - 3c_{30}c_{34} + 4c_{32}c_{34}) + c_{12}c_{30}(3c_{30} - c_{34}) \right] - c_{32}q^2(c_{10} - c_{12})(c_{30} - 3c_{34}) \right. \\ & \left. + m_B^2 (c_{10}c_{32}(c_{30} - 4c_{34}) + c_{12}c_{30}c_{34}) - m_b^2(c_{10} + 3c_{12}) + 3c_{10}m_b m_B(c_{32} + c_{34}) \right), \end{aligned}$$

$$\bar{C}_1^{(1,\Phi)} = -4(c_{10} + 3c_{12} + 2c_{30} - 6(c_{32} + c_{34})),$$

$$\begin{aligned} \bar{C}_0^{(2,\Phi)} = & 8 \left( s \left\{ q^2 [\hat{\omega}(c_{10} - c_{12})(c_{30} - c_{32})(c_{30} - c_{34}) - 3c_{10}c_{30}c_{32} - 2c_{10}c_{30}c_{34} + 3c_{10}c_{32}c_{34} \right. \right. \\ & \left. \left. + 4c_{12}c_{30}^2 - c_{12}c_{30}c_{32} - 2c_{12}c_{30}c_{34} + c_{12}c_{32}c_{34}] - (\hat{\omega} - 1) \left[ c_{10}(-m_B^2(c_{30}^2\hat{\omega} \right. \right. \right. \\ & \left. \left. \left. + c_{30}c_{32}(2\hat{\omega} - 3) + c_{30}c_{34}(3\hat{\omega} - 2) - 2c_{32}c_{34}(\hat{\omega} - 1)) + m_b m_B(2\hat{\omega}(2c_{32} + c_{34}) \right. \right. \right. \end{aligned}$$

$$\begin{aligned}
& -3(c_{32} + c_{34})) + m_b^2) + c_{12}(c_{30}m_B^2(3c_{30}\hat{\omega} - 4c_{30} + c_{34}\hat{\omega} + c_{34}) \\
& - 2m_b m_B(\hat{\omega} - 1)(2c_{32} + c_{34}) - m_b^2)] \Big\} + q^2 \Big[ c_{10}c_{32}m_B(\omega(-c_{30}m_B(\hat{\omega} - 2) \\
& + 2m_b\hat{\omega} + m_b) + c_{34}m_B(-3(\hat{\omega} - 1)\hat{\omega} - 4)) - c_{10}m_b\hat{\omega}(c_{34}m_B(1 - 4\hat{\omega}) + m_b) \\
& + c_{12}m_B^2(c_{32}(\hat{\omega} - 1)(c_{30}\hat{\omega} + c_{34}(3\hat{\omega} - 2)) + c_{30}c_{34}\omega) - 2c_{12}m_b m_B(\hat{\omega} - 1) \\
& (c_{32}(\hat{\omega} + 2) + 2c_{34}\hat{\omega} + c_{34}) + c_{12}m_b^2(\omega - 4) \Big] + c_{32}q^4(c_{10} - c_{12})(c_{34}(\hat{\omega} + 2) \\
& - c_{30}\hat{\omega}) + c_{30}(\hat{\omega} - 1)s^2(c_{10} - c_{12})(c_{30} - c_{34}) + m_B^2(\hat{\omega} - 1) \Big[ c_{10}c_{32}m_B \\
& (\omega(c_{30}m_B + m_b) + 2c_{34}m_B(\hat{\omega} - 1)) - c_{10}m_b\hat{\omega}(c_{34}m_B + m_b) \\
& + c_{12}c_{30}c_{34}m_B^2\hat{\omega} - 2c_{12}m_b m_B(\hat{\omega} - 1)(2c_{32} + c_{34}) + c_{12}m_b^2(3\hat{\omega} - 4) \Big] \Big), \\
\bar{C}_1^{(2, \Phi)} = & 4 \Big( q^2(\hat{\omega}(c_{10} - c_{12} + 2c_{30} + c_{32} - 2c_{34}) + 4c_{12} - 7c_{32} - 4c_{34}) + (\hat{\omega} - 1)s(c_{10} \\
& - c_{12} + c_{32} - 2c_{34}) + m_B(\hat{\omega} - 1)(m_B(\hat{\omega}(c_{10} + 2c_{30} + 6(c_{32} + c_{34}))) \\
& + c_{12}(4 - 3\hat{\omega}) - 7c_{32} - 4c_{34}) - 6m_b\hat{\omega}) \Big).
\end{aligned}$$

•  $\bar{B}_i^{(j, \phi/\Phi)}$ :

The coefficients used in the  $I^{(B3)}$  function ( $\bar{B}$ ) are given below:

$$\begin{aligned}
\bar{B}_0^{(0, \phi)} &= -12 m_B^3 \hat{m}_b^2 x^2 (\hat{\omega} - 1) (2\hat{\omega} - 1), & \bar{B}_1^{(0, \phi)} &= -12 m_B (\hat{\omega} - 1) (2\hat{\omega} - 1), \\
\bar{B}_0^{(1, \Phi)} &= \bar{B}_1^{(1, \Phi)} = 0, & \bar{B}_0^{(2, \Phi)} &= 24 m_B^2 \hat{m}_b^2 x^2 (2\hat{\omega} - 1), \\
\bar{B}_1^{(2, \Phi)} &= 24 (2\hat{\omega} - 1), & \bar{B}_0^{(3, \Phi)} &= 48 m_B^4 \hat{m}_b^2 x^2 (\hat{\omega} - 1)^2 \hat{\omega}, \\
\bar{B}_1^{(3, \Phi)} &= 48 m_B^2 (\hat{\omega} - 1)^2 \hat{\omega}, & \bar{B}_0^{(4, \Phi)} &= 24 m_B^4 \hat{m}_b^2 x^2 (\hat{\omega} - 1)^2 (2\hat{\omega} - 1), \\
\bar{B}_1^{(4, \Phi)} &= 24 m_B^2 (\hat{\omega} - 1)^2 (2\hat{\omega} - 1).
\end{aligned}$$

### 1.3 Diagram in Fig 1C

This section provides the explicit coefficient functions  $D_i^{(j, \phi/\Phi)}$ ,  $B_i^{(j, \phi/\Phi)}$ ,  $A_i^{(j, \phi/\Phi)}$ , and  $C_i^{(j, \phi/\Phi)}$  that enter the invariant amplitudes the invariant amplitudes  $I^{(C1)}$ - $I^{(C4)}$ . The  $\phi(\Phi)$  denote the terms multiplying, respectively, the twist-two(three)  $B$ -meson distribution amplitudes. All coefficients depend on the external and kinematic variables as  $X_i^{(j, \phi/\Phi)} =$

$X_i^{(j,\phi/\Phi)}(s, q^2, m_B, m_b, \hat{\omega}; x_1, x_2, x_3)$ ,  $\hat{m}_b = \frac{m_b}{m_B}$ ,  $\hat{\omega} = \frac{\omega}{m_B}$ . A prime on  $\tilde{X}$  indicates a derivative with respect to the dispersion variable  $s$ .

•  $D_i^{(j,\phi/\Phi)}$ :

The coefficients used in the  $I^{(C1)}$  function ( $D$ ) are given below:

$$\begin{aligned} D_0^{(0,\phi)}(s, q^2) = & -4 m_B \left( \hat{\omega} \left( x_3 q^2 [\hat{\omega}(x_2 + x_3 - 1)(6\hat{m}_b(x_2 + x_3 - 1) - 3x_2 - 3x_3 + 4) \right. \right. \\ & - (x_3 - 1)((6\hat{m}_b - 3)x_2 + 6\hat{m}_b x_3 - 3x_3 + 1)] + m_B^2 [3(2\hat{m}_b - 1)\hat{\omega}^2 \\ & (x_2 + x_3 - 1)^2(x_2 + x_3) - \hat{\omega}(x_2 + x_3 - 1)(3(2\hat{m}_b - 1)x_2(2x_3 - 1) \\ & + 2x_3(6\hat{m}_b x_3 - 3\hat{m}_b - 3x_3 + 2)) + (x_3 - 1)x_3((6\hat{m}_b - 3)x_2 + 6\hat{m}_b x_3 \\ & \left. \left. - 3x_3 + 1) \right] \right) - x_3 s (\hat{\omega}(x_2 + x_3 - 1) - x_3 + 1) (\hat{\omega}(6\hat{m}_b(x_2 - 1) - 3x_2 \\ & + 2) + 3(2\hat{m}_b - 1)x_3(\hat{\omega} - 1)) \Big), \end{aligned}$$

$$D_1^{(0,\phi)}(s, q^2) = -6 m_B (2\hat{m}_b - 1) ((3x_2 - 4)\hat{\omega} + 3x_3(\hat{\omega} - 1) + 2),$$

$$D_2^{(0,\phi)}(s, q^2) = 0,$$

$$\begin{aligned} D_0^{(1,\phi)}(s, q^2) = & 8 \left( - (4\hat{m}_b - 1) x_3 s (\hat{\omega}(x_2 + x_3 - 1) - x_3 + 1) + x_3 q^2 ((4\hat{m}_b - 3)\hat{\omega}(x_2 + x_3 - 1) \right. \\ & - 2(\hat{m}_b - 1)(x_3 - 1)) + m_B^2 (\hat{\omega}(x_2 + x_3 - 1) - x_3 + 1) (3(2\hat{m}_b - 1)\hat{\omega}(x_2 + x_3) \\ & \left. - 2(\hat{m}_b - 1)x_3) \right), \end{aligned}$$

$$D_1^{(1,\phi)}(s, q^2) = 12 (2\hat{m}_b - 1),$$

$$D_2^{(1,\phi)}(s, q^2) = 0,$$

$$\begin{aligned} D_0^{(2,\phi)}(s, q^2) = & 24 \left( x_3 s (\hat{\omega}(-2\hat{m}_b x_2 + 2\hat{m}_b + x_2) + x_3(-2\hat{m}_b \hat{\omega} + 2\hat{m}_b + \hat{\omega} - 1)) + x_3 \hat{\omega} q^2 (2\hat{m}_b(x_2 \right. \\ & + x_3 - 1) - x_2 - x_3 + 2) + m_B^2 \hat{\omega} ((2\hat{m}_b - 1)\hat{\omega}(x_2 + x_3 - 1)(x_2 + x_3) \\ & \left. + x_3(-2\hat{m}_b x_2 - 2\hat{m}_b x_3 + x_2 + x_3 - 1)) \right), \end{aligned}$$

$$D_1^{(2,\phi)}(s, q^2) = 24 (2\hat{m}_b - 1),$$



$$D_2^{(2,\phi)}(s, q^2) = 0,$$

$$\begin{aligned}
D_0^{(3,\phi)}(s, q^2) = & -8 \left( x_3 s \left[ x_3 q^2 \left( \hat{\omega} (2\hat{m}_b(5x_2x_3 - 3x_2 + 5x_3^2 - 7x_3 + 2) - 6x_3(x_2 + x_3) + 3x_2 + 10x_3 - 4) \right. \right. \right. \\
& - 4(2\hat{m}_b - 1)\hat{\omega}^2(x_2 + x_3 - 1)^2 - 2(\hat{m}_b - 1)(x_3 - 1)x_3 \Big) - 2m_B^2(\hat{\omega}(x_2 + x_3 - 1) - x_3 \\
& + 1) \left( \hat{\omega}^2(x_2 + x_3 - 1)(\hat{m}_b(5x_2 + 5x_3 - 3) - 2x_2 - 2x_3 + 1) + x_3\hat{\omega}(\hat{m}_b(-6x_2 - 6x_3 + 4) \right. \\
& + 3(x_2 + x_3 - 1)) + (\hat{m}_b - 1)x_3^2 \Big) \Big] + \hat{\omega} \left[ x_3 q^2 \left( x_3 q^2 (\hat{\omega}(x_2 + x_3 - 1)(4\hat{m}_b(x_2 + x_3 - 1) \right. \right. \\
& - 3x_2 - 3x_3 + 4) - 2(\hat{m}_b - 1)(x_3 - 1)(x_2 + x_3)) + m_B^2 \left( 2\hat{\omega}^2(x_2 + x_3 - 1)^2 (\hat{m}_b(5x_2 \right. \\
& + 5x_3 - 3) - 3x_2 - 3x_3 + 2) - \hat{\omega}(x_2 + x_3 - 1) \left( x_2(2(7\hat{m}_b - 5)x_3 - 8\hat{m}_b + 5) \right. \\
& + 2x_3(7\hat{m}_bx_3 - 6\hat{m}_b - 5x_3 + 5) - 1) + 4(\hat{m}_b - 1)(x_3 - 1)x_3(x_2 + x_3) \Big) \Big) \\
& + m_B^4(\hat{\omega}(x_2 + x_3 - 1) - x_3 + 1) \left( 2(\hat{m}_b - 1)x_3^2(x_2 + x_3) + 3(2\hat{m}_b - 1)\hat{\omega}^2(x_2 + x_3 - 1)^2 \right. \\
& (x_2 + x_3) - x_3\hat{\omega}(x_2 + x_3 - 1)((8\hat{m}_b - 5)x_2 + 8\hat{m}_bx_3 - 5x_3 + 1) \Big) \Big] + x_3^2 s^2 \\
& \left. \left( \hat{\omega}(x_2 + x_3 - 1) - x_3 + 1) (4\hat{m}_b(x_2 - 1)\hat{\omega} + (4\hat{m}_b - 1)x_3(\hat{\omega} - 1) - x_2\hat{\omega}) \right) \right),
\end{aligned}$$

$$\begin{aligned}
D_1^{(3,\phi)}(s, q^2) = & -4 \left( -s \left( x_3(\hat{m}_b(16x_2\hat{\omega} - 15\hat{\omega} + 7) + \hat{\omega}(2x_2(\hat{\omega} - 3) - 3\hat{\omega} + 3) - 2) \right. \right. \\
& + (x_2 - 2)\hat{\omega}(\hat{m}_b + (x_2 - 1)\hat{\omega} + 1) + x_3^2(\hat{\omega} - 1)(16\hat{m}_b + \hat{\omega} - 5) \Big) \\
& + q^2 \left( \hat{\omega}(\hat{m}_b(16x_2x_3 + x_2 + x_3(16x_3 - 15) - 2) - 12x_3(x_2 + x_3) + x_2 + 15x_3 + 2) \right. \\
& - 3(\hat{m}_b - 1)x_3(2x_3 - 1) + \hat{\omega}^2(x_2 + x_3 - 2)(x_2 + x_3 - 1) \Big) + 2\hat{\omega}^2(x_2 + x_3 - 1) \\
& \left( m_B^2(\hat{m}_b(11x_2 + 11x_3 - 8) - 5x_2 - 5x_3 + 3) + 2(8\hat{m}_b(x_2 + x_3 - 1) - 5x_2 \right. \\
& - 5x_3 + 6) \Big) + \hat{\omega} \left( -\hat{m}_b(m_B^2(x_2(28x_3 - 11) + x_3(28x_3 - 33) + 6) + 40x_3(x_2 + x_3) \right. \\
& - 4(7x_2 + 15x_3 - 6)) + m_B^2(4x_2(4x_3 - 1) + x_3(16x_3 - 21)) + 26x_3(x_2 + x_3)
\end{aligned}$$

$$-20x_2 - 42x_3 + 20) + x_3(3m_B^2(\hat{m}_b - 1)(2x_3 - 1) + 2\hat{m}_b(6x_3 - 7) - 8x_3 + 10)) ,$$

$$D_2^{(3,\phi)}(s, q^2) = -12(2\hat{m}_b - 1) ,$$

$$\begin{aligned} D_0^{(4,\phi)}(s, q^2) = & 8 \left( s \left( (x_3 - 1)x_3 q^2 (4(2\hat{m}_b - 1)\hat{\omega}^2(x_2 + x_3 - 1)^2 + \hat{\omega}(2\hat{m}_b(x_2(3 - 5x_3) \right. \right. \\ & + (7 - 5x_3)x_3 - 2) + 6x_3(x_2 + x_3) - 3x_2 - 10x_3 + 4) + 2(\hat{m}_b - 1)(x_3 - 1)x_3) \\ & + m_B^2(\hat{\omega}(x_2 + x_3 - 1) - x_3 + 1) \left[ x_3\hat{\omega}(3(2x_3 - 1)(x_2 + x_3 - 1) - 2\hat{m}_b(6x_2x_3 \right. \\ & - 3x_2 + 6x_3^2 - 7x_3 + 1)) + \hat{\omega}^2(x_2 + x_3 - 1)(x_2(10\hat{m}_bx_3 - 4\hat{m}_b - 4x_3 + 1) \\ & + x_3(10\hat{m}_b(x_3 - 1) - 4x_3 + 3)) + 2(\hat{m}_b - 1)(x_3 - 1)x_3^2 \Big] + \hat{\omega} \left( m_B^2 q^2 \left[ -\hat{\omega}^2 \right. \right. \\ & (x_2 + x_3 - 1)^2(x_2(10\hat{m}_bx_3 - 4\hat{m}_b - 6x_3 + 3) + x_3(10\hat{m}_b(x_3 - 1) - 6x_3 + 7)) \\ & + (x_3 - 1)\hat{\omega}(x_2 + x_3 - 1) \left( 2x_2(7\hat{m}_bx_3 - \hat{m}_b - 5x_3 + 1) + x_3(2(7\hat{m}_b - 5)x_3 - 6\hat{m}_b + 7) \right) \\ & - 4(\hat{m}_b - 1)x_3(x_3 - 1)^2(x_2 + x_3) \Big] - (x_3 - 1)x_3 q^4 (\hat{\omega}(x_2 + x_3 - 1)(4\hat{m}_b(x_2 + x_3 - 1) \\ & - 3x_2 - 3x_3 + 4) - 2(\hat{m}_b - 1)(x_3 - 1)(x_2 + x_3)) - m_B^4(\hat{\omega}(x_2 + x_3 - 1) \\ & - x_3 + 1) \left( 3(2\hat{m}_b - 1)\hat{\omega}^2(x_2 + x_3 - 1)^2(x_2 + x_3) - \hat{\omega}(x_2 + x_3 - 1)(x_2(8\hat{m}_bx_3 \right. \\ & - 2\hat{m}_b - 5x_3 + 2) + x_3(8\hat{m}_bx_3 - 2\hat{m}_b - 5x_3 + 3)) + 2(\hat{m}_b - 1)(x_3 - 1)x_3(x_2 + x_3) \Big) \Big) \\ & \left. - (x_3 - 1)x_3 s^2 (\hat{\omega}(x_2 + x_3 - 1) - x_3 + 1) (4\hat{m}_b(x_2 - 1)\hat{\omega} + (4\hat{m}_b - 1)x_3(\hat{\omega} - 1) - x_2\hat{\omega}) \right) , \end{aligned}$$

$$\begin{aligned} D_1^{(4,\phi)}(s, q^2) = & -4 \left( -s \left( \hat{m}_b\hat{\omega}(2x_2(8x_3 - 5) + 2x_3(8x_3 - 13) + 11) - 2\hat{m}_b(x_3(8x_3 - 9) + 4) \right. \right. \\ & + \hat{\omega}^2(x_2 + x_3 - 2)(x_2 + x_3 - 1) + x_3\hat{\omega}(-6x_2 - 6x_3 + 5) + 3(x_2 - 1)\hat{\omega} \\ & + x_3(5x_3 - 4) + 2) + q^2 \left( \hat{\omega}(\hat{m}_b(2x_2(8x_3 - 5) + 2x_3(8x_3 - 13) + 11) \right. \\ & - 12x_3(x_2 + x_3) + 9x_2 + 23x_3 - 9) - 2(\hat{m}_b - 1)(x_3 - 1)(3x_3 - 2) + \hat{\omega}^2(x_2 \\ & \left. \left. + x_3 - 2)(x_2 + x_3 - 1) \right) + 2\hat{\omega}^2(x_2 + x_3 - 1) \left( m_B^2(\hat{m}_b(11x_2 + 11x_3 - 8) \right. \right. \end{aligned}$$

$$\begin{aligned}
& -5x_2 - 5x_3 + 3) + 2(8\hat{m}_b(x_2 + x_3 - 1) - 5x_2 - 5x_3 + 6)) + \hat{\omega} \left( m_B^2 (\hat{m}_b (x_2 (18 \right. \\
& \quad \left. - 28x_3) + 4(10 - 7x_3)x_3 - 17) + 16x_3(x_2 + x_3) - 11x_2 - 28x_3 + 11) \right. \\
& \quad \left. + 2(-2\hat{m}_b(2x_2(5x_3 - 3) + 2x_3(5x_3 - 7) + 5) + 13x_3(x_2 + x_3) - 8x_2 - 19x_3 + 8) \right) \\
& \quad \left. + 2(x_3 - 1)(m_B^2(\hat{m}_b - 1)(3x_3 - 2) + 6\hat{m}_b x_3 - 4x_3) \right),
\end{aligned}$$

$$D_2^{(4,\phi)}(s, q^2) = -12(2\hat{m}_b - 1).$$

•  $B_i^{(j,\phi/\Phi)}$ :

The coefficients used in the  $I^{(C2)}$  function ( $B$ ) are given below with the following shorthand parameter combinations:

$$\begin{aligned}
a_1 &= -(x_1 + x_2 + x_3), & a_2 &= x_2 + x_3, & a_3 &= x_3, \\
a_4 &= 1 - (x_1 + x_2 + x_3), & a_5 &= x_2 + x_3 - 1, & a_6 &= x_3 - 1. \\
a_{12} &= a_1 \omega + a_2, & a_{13} &= a_1 \omega + a_3, & a_{42} &= a_4 \omega + a_2, \\
a_{43} &= a_4 \omega + a_3, & a_{45} &= a_4 \omega + a_5, & a_{46} &= a_4 \omega + a_6.
\end{aligned}$$

$$\begin{aligned}
B_0^{(0,\phi)}(s, q^2) &= 12 m_B \left( a_{45} s [a_{12} a_{43} (a_{42} + a_{45}) + a_{12} a_{46} (a_{42} - a_{43}) - a_{13} a_{42} (a_{43} + a_{45})] \right. \\
& \quad \left. + a_{43} q^2 [-a_{12} a_{46} (a_{43} + a_{45}) + a_{13} a_{42} (a_{46} - a_{45}) + a_{13} a_{45} (a_{43} + a_{46})] \right. \\
& \quad \left. + a_{43} a_{45} m_B^2 (a_{12} a_{46} + a_{13} a_{42}) \right),
\end{aligned}$$

$$B_1^{(0,\phi)}(s, q^2) = -6 m_B (a_{12} a_{46} + a_{13} a_{42} - 2a_{42} (a_{43} + a_{46}) - 2a_{45} (2a_{43} + a_{46})),$$

$$B_2^{(0,\phi)}(s, q^2) = 0,$$

$$\begin{aligned}
B_0^{(1,\Phi)}(s, q^2) &= 8 \left( (a_{12} - a_{13}) [a_{45} s (2a_{43} + a_{45} + a_{46}) - q^2 (a_{43} (a_{45} + a_{46}) + 2a_{45} a_{46})] \right. \\
& \quad \left. + a_{45} m_B^2 (a_{12} (a_{43} + 2a_{46}) + a_{13} (2a_{43} + a_{46})) \right),
\end{aligned}$$

$$B_1^{(1,\Phi)}(s, q^2) = 4 (a_{12} - a_{13} + 3a_{43} + 4a_{45} + 3a_{46}),$$

$$B_2^{(1,\Phi)}(s, q^2) = 0,$$

$$\begin{aligned}
B_0^{(2,\Phi)}(s, q^2) = & 8 \left( s \left[ a_{12} a_{42} (a_{45} + 3a_{46}) + a_{12} a_{43} (a_{45} - a_{46}) - 2a_{13} a_{42} (a_{45} + a_{46}) \right] \right. \\
& + q^2 \left[ -4a_{12} a_{43} a_{46} + a_{13} a_{42} (a_{46} - a_{45}) + a_{13} a_{43} (a_{45} + 3a_{46}) \right] + m_B^2 (a_{12} a_{43} a_{46} \\
& \left. + a_{13} a_{42} (a_{45} + 2a_{46})) \right)
\end{aligned}$$

$$B_1^{(2,\Phi)}(s, q^2) = -4(2a_{12} - 3a_{42} - 3a_{43} - 2a_{45} - 6a_{46}),$$

$$B_2^{(2,\Phi)}(s, q^2) = 0,$$

$$B_0^{(3,\Phi)}(s, q^2) = 24 \left( (a_{12} - a_{13})(a_{43} + a_{45})(a_{42} s - a_{43} q^2) + a_{43} m_B^2 (a_{12} a_{45} + a_{13} a_{42}) \right),$$

$$B_1^{(3,\phi)}(s, q^2) = -12(a_{12} - a_{13} - 2(a_{42} + a_{43} + a_{45})),$$

$$B_2^{(3,\phi)}(s, q^2) = 0,$$

$$\begin{aligned}
B_0^{(4,\Phi)}(s, q^2) = & -8 \left( s \left[ a_{45} m_B^2 (a_{12} a_{43} (a_{42}^2 + 2a_{42} (a_{43} + a_{45}) + a_{43} a_{45}) + 2a_{12} a_{46} (a_{42} - a_{43}) (a_{42} + a_{43}) \right. \right. \\
& + a_{13} a_{42} (a_{42} (a_{43} - a_{45}) - 2a_{43} (2a_{43} + a_{45}))) - q^2 (a_{42} - a_{43}) (a_{12} a_{46} (a_{43} (a_{42} + a_{43}) \\
& + 2a_{42} a_{45}) + a_{12} a_{43} a_{45} (a_{42} + a_{43} + 2a_{45}) - a_{13} (2a_{42} a_{43} a_{46} + a_{42} a_{45} (a_{45} + a_{46}) \\
& + 2a_{43}^2 a_{45} + a_{43} a_{45} (a_{45} + a_{46}))) \left. \right] + a_{43} q^2 \left[ q^2 (a_{43} - a_{42}) (-2a_{12} a_{46} (a_{43} + a_{45}) \right. \\
& + a_{13} a_{46} (a_{42} + a_{43} + 2a_{45}) + a_{13} a_{45} (a_{43} - a_{42})) + m_B^2 (a_{46} (a_{12} a_{45} (a_{43} - 4a_{42}) \\
& - a_{12} a_{43} (2a_{42} + a_{43}) + a_{13} (a_{42}^2 + 2a_{42} (a_{43} + a_{45}) + a_{43} a_{45})) \\
& \left. \left. - 2a_{13} a_{45} (a_{42} - a_{43}) (a_{42} + a_{43})) \right] + a_{45} s^2 (a_{42} - a_{43}) (a_{12} a_{42} (2a_{43} + a_{45} + a_{46}) \right. \\
& + a_{12} a_{43} (a_{45} - a_{46}) - 2a_{13} a_{42} (a_{43} + a_{45})) + a_{43} a_{45} m_B^4 (a_{12} a_{46} (2a_{42} + a_{43}) \\
& \left. \left. + a_{13} a_{42} (a_{42} + 2a_{43})) \right) \right),
\end{aligned}$$

$$\begin{aligned}
B_1^{(4,\Phi)}(s, q^2) = & -4 \left( s \left[ a_{12} (a_{42}^2 + 2a_{42} (a_{43} + 2a_{45} + a_{46}) + a_{43} (a_{45} - a_{46}) + a_{45} (a_{45} + a_{46})) \right. \right. \\
& - a_{13} (2a_{42}^2 + a_{42} (a_{43} + 4a_{45} + 2a_{46}) + a_{45} (a_{45} + a_{46})) + 3a_{42}^2 a_{43} + 2a_{42}^2 a_{46} \\
& \left. \left. - 3a_{42} a_{43}^2 + 6a_{42} a_{43} a_{45} + 2a_{42} a_{45}^2 - 8a_{43}^2 a_{45} - 2a_{43} a_{45}^2 \right] + q^2 \left[ 2a_{46} (-a_{45} (a_{12} \right. \right.
\end{aligned}$$

$$\begin{aligned}
& + a_{42} - a_{43}) + a_{12}a_{42} - 2a_{12}a_{43} - 2a_{42}^2 + a_{43}^2) + a_{43}(-3(a_{12}a_{43} + a_{42}^2 - a_{42}a_{43}) \\
& - 2a_{45}(2a_{12} + a_{42} - 2a_{43})) + a_{13}(a_{42}^2 - a_{42}(a_{43} + 2a_{45}) + 3a_{43}^2 + 5a_{43}a_{45} + 3a_{43}a_{46} \\
& + 2a_{45}a_{46})) + m_B^2[a_{12}a_{46}(-2a_{42} + a_{43} + 2a_{45}) + 2a_{43}a_{45}(2a_{12} + a_{42} + 4a_{43}) \\
& + a_{13}(-a_{42}^2 + a_{42}(a_{43} + 2(a_{45} + a_{46})) + a_{45}a_{46}) + 3a_{42}a_{43}(a_{42} + a_{43}) \\
& + 2a_{42}a_{46}(2a_{42} + a_{45})) + 2a_{45}(a_{43}(a_{12} + 3a_{13} + 4a_{42}) + a_{42}(a_{42} - 2a_{13}) - a_{43}^2) \\
& + 2a_{46}(-3a_{12}a_{43} + a_{13}a_{43} + 4a_{45}(a_{42} + a_{43}) + 4a_{42}a_{43}))],
\end{aligned}$$

$$B_2^{(4,\Phi)}(s, q^2) = 4(2a_{12} - 4a_{42} - 3a_{43} - 4a_{45} - 3a_{46}),$$

$$\begin{aligned}
B_0^{(5,\Phi)}(s, q^2) = & -8\left(s\left\{q^2(a_{43} - a_{45})[a_{12}a_{46}(a_{43}(a_{42} + a_{43}) + 2a_{42}a_{45}) + a_{12}a_{43}a_{45}(a_{42} + a_{43} + 2a_{45}) \right. \right. \\
& - a_{13}(2a_{42}a_{43}a_{46} + a_{42}a_{45}(a_{45} + a_{46}) + 2a_{43}^2a_{45} + a_{43}a_{45}(a_{45} + a_{46}))] \\
& + a_{45}m_B^2[a_{12}a_{46}(a_{42}(a_{43} + 2a_{45}) - a_{43}(2a_{43} + a_{45})) + a_{12}a_{43}(a_{42}(2a_{43} + a_{45}) \\
& + a_{45}(a_{43} + 2a_{45})) - a_{13}a_{42}(4a_{43}^2 + a_{43}a_{45} + a_{45}^2)]\left. \right\} + a_{43}q^2[q^2(a_{43} - a_{45})(-2a_{12}a_{46}(a_{43} \\
& + a_{45}) + a_{13}a_{46}(a_{42} + a_{43} + 2a_{45}) + a_{13}a_{45}(a_{43} - a_{42})) + m_B^2(-a_{12}a_{46}(a_{43}^2 \\
& + a_{43}a_{45} + 4a_{45}^2) + a_{13}a_{46}(a_{42}(2a_{43} + a_{45}) + a_{45}(a_{43} + 2a_{45})) - a_{13}a_{42}a_{45}(a_{43} \\
& + 2a_{45}) + a_{13}a_{43}a_{45}(2a_{43} + a_{45}))] + a_{45}s^2(a_{45} - a_{43})(a_{12}a_{42}(2a_{43} + a_{45} + a_{46}) \\
& + a_{12}a_{43}(a_{45} - a_{46}) - 2a_{13}a_{42}(a_{43} + a_{45})) + a_{43}a_{45}m_B^4(a_{12}a_{46}(a_{43} + 2a_{45}) \\
& + a_{13}a_{42}(2a_{43} + a_{45}))),
\end{aligned}$$

$$\begin{aligned}
B_1^{(5,\Phi)}(s, q^2) = & -4\left(q^2[2a_{46}(-2a_{12}a_{43} + a_{43}(a_{42} + a_{43}) - a_{42}a_{45} - 2a_{45}^2) - a_{43}(a_{45}(4a_{12} + a_{42} \right. \\
& - 4a_{43}) + 3a_{43}(a_{12} - a_{42}) + 4a_{45}^2) + a_{13}(-a_{42}(a_{43} + a_{45} - a_{46}) + 3a_{43}^2 + 5a_{43}a_{45} \\
& + 3a_{43}a_{46} + a_{45}a_{46})] + s[a_{12}(a_{42}(2a_{43} + 5a_{45} + 3a_{46}) + a_{45}(a_{43} + a_{45}) - a_{43}a_{46}) \\
& - a_{13}(a_{42}(a_{43} + 6a_{45} + 2a_{46}) + a_{45}(a_{45} + a_{46})) - 3a_{42}a_{43}^2 + a_{42}a_{43}a_{45} - 8a_{43}^2a_{45} \\
& + 6a_{43}a_{45}^2 + 2a_{45}^3 + 2a_{45}^2a_{46}] + m_B^2[4a_{43}a_{45}(a_{12} + 2a_{43} + a_{45}) + a_{12}a_{43}a_{46}
\end{aligned}$$

$$\begin{aligned}
& + a_{13}a_{42}(a_{43} + a_{45}) + a_{13}a_{46}(2a_{42} + a_{45}) + a_{42}a_{43}(3a_{43} + a_{45}) + 2a_{45}a_{46}(a_{42} + 2a_{45})] \\
& + 2a_{46}(-3a_{12}a_{43} + a_{13}a_{43} + 4a_{45}(a_{42} + a_{43}) + 4a_{42}a_{43}) + 2a_{45}(a_{43}(a_{12} + 3a_{42} - a_{43}) \\
& + a_{13}(3a_{43} - 2a_{42}) + a_{45}(a_{42} + a_{43}))) ,
\end{aligned}$$

$$B_2^{(5,\Phi)}(s, q^2) = 4(2a_{12} - 3a_{42} - 3a_{43} - 5a_{45} - 3a_{46}) ,$$

$$\begin{aligned}
B_0^{(6,\Phi)}(s, q^2) = & -8 \left( s \left[ a_{45}m_B^2 (a_{12}(2a_{42}a_{46}(a_{43} + a_{45}) + a_{43}a_{45}(a_{42} + 2a_{45}) + a_{46}^2(a_{42} - 2a_{43})) \right. \right. \\
& + a_{13}a_{42}(a_{45}(a_{43} - a_{45}) - 2a_{46}(2a_{43} + a_{45}))) - q^2(a_{45} - a_{46})(a_{12}a_{46}(a_{43}(a_{42} + a_{43}) \\
& + 2a_{42}a_{45}) + a_{12}a_{43}a_{45}(a_{42} + a_{43} + 2a_{45}) - a_{13}(2a_{42}a_{43}a_{46} + a_{42}a_{45}(a_{45} + a_{46}) \\
& + 2a_{43}^2a_{45} + a_{43}a_{45}(a_{45} + a_{46}))) \left. \right] + a_{43}q^2 \left[ m_B^2(a_{46}^2(a_{45}(a_{12} + a_{13}) - a_{12}a_{43} + 2a_{13}a_{42}) \right. \\
& + 2a_{45}a_{46}(a_{13}(a_{43} + a_{45}) - a_{12}(a_{43} + 2a_{45}))) + a_{13}a_{45}^2(a_{43} - 2a_{42})) - q^2(a_{45} - a_{46}) \\
& \left. \left( -2a_{12}a_{46}(a_{43} + a_{45}) + a_{13}a_{46}(a_{42} + a_{43} + 2a_{45}) + a_{13}a_{45}(a_{43} - a_{42}) \right) \right] \\
& + a_{45}s^2(a_{45} - a_{46})(a_{12}a_{42}(2a_{43} + a_{45} + a_{46}) + a_{12}a_{43}(a_{45} - a_{46}) - 2a_{13}a_{42}(a_{43} + a_{45})) \\
& \left. + a_{43}a_{45}m_B^4(a_{12}a_{46}(2a_{45} + a_{46}) + a_{13}a_{42}(a_{45} + 2a_{46})) \right) ,
\end{aligned}$$

$$\begin{aligned}
B_1^{(6,\Phi)}(s, q^2) = & -4 \left( q^2 \left( -a_{12}(3a_{43}^2 + 2a_{43}(2a_{45} + a_{46}) + 2a_{46}^2) + a_{13}(-a_{42}a_{45} + 3a_{43}^2 + 5a_{43}a_{45} \right. \right. \\
& + 2a_{43}a_{46} + a_{45}a_{46} + a_{46}^2) + a_{46}(a_{42}a_{43} - 2a_{42}a_{45} - 4a_{45}^2) + 2a_{46}^2(2a_{42} + a_{43} + 2a_{45}) \\
& - a_{43}a_{45}(a_{42} + 4a_{45})) + s \left( a_{12}(a_{42}(3a_{43} + 5a_{45} + 2a_{46}) + a_{45}(a_{43} + a_{45}) - 2a_{43}a_{46} \right. \\
& + a_{46}^2) - a_{13}(3a_{42}(a_{43} + 2a_{45}) + a_{45}(a_{45} + a_{46})) - a_{43}a_{46}(a_{42} + 6a_{45}) + a_{45}(a_{42}a_{43} \\
& + 2a_{45}(4a_{43} + a_{45})) - 2a_{46}^2(a_{42} + a_{45})) + m_B^2(a_{46}(2a_{12}a_{43} + a_{42}a_{43} + 2a_{42}a_{45} \\
& + 6a_{43}a_{45} + 4a_{45}^2) + a_{43}a_{45}(4a_{12} + a_{42} + 4a_{45}) + a_{46}^2(2(a_{42} + a_{45}) - a_{12}) \\
& + a_{13}(a_{42}(3a_{43} + a_{45}) + a_{45}a_{46})) + 2(a_{46}(-3a_{12}a_{43} + a_{13}a_{43} + 3a_{45}(a_{42} + a_{43}) + 4a_{42}a_{43}) \\
& \left. \left. + a_{45}(a_{12}a_{43} - 2a_{13}a_{42} + 3a_{13}a_{43} + a_{45}(a_{42} + a_{43}) + 4a_{42}a_{43})) \right) \right) ,
\end{aligned}$$

$$B_2^{(6,\Phi)}(s, q^2) = 4(2a_{12} - 3a_{42} - 4a_{43} - 5a_{45} - 2a_{46}) .$$

•  $A_i^{(j,\phi/\Phi)}$ :

The coefficients used in the  $I^{(C3)}$  function ( $A$ ) are given below with the following shorthand parameter combinations:

$$\tilde{a}_1 = x_1 + x_2 + x_3, \quad \tilde{a}_2 = x_3, \quad \tilde{a}_3 = x_2 + x_3$$

$$\tilde{a}_4 = 1 - (x_1 + x_2 + x_3), \quad \tilde{a}_5 = x_2 + x_3 - 1, \quad \tilde{a}_6 = x_3 - 1 .$$

$$\tilde{a}_{12} = \tilde{a}_1 \hat{\omega} + \tilde{a}_2, \quad \tilde{a}_{13} = \tilde{a}_1 \hat{\omega} + \tilde{a}_3, \quad \tilde{a}_{42} = \tilde{a}_4 \hat{\omega} + \tilde{a}_2$$

$$\tilde{a}_{43} = \tilde{a}_4 \hat{\omega} + \tilde{a}_3, \quad \tilde{a}_{45} = \tilde{a}_4 \hat{\omega} + \tilde{a}_5, \quad \tilde{a}_{46} = \tilde{a}_4 \hat{\omega} + \tilde{a}_6 .$$

$$\begin{aligned} A_0^{(0,\phi)}(s, q^2) = & 12m_B \left( \tilde{a}_{42} s \left[ \tilde{a}_{12} \tilde{a}_{45} (\tilde{a}_{42} - \tilde{a}_{43}) + \tilde{a}_{12} \tilde{a}_{46} (\tilde{a}_{43} + \tilde{a}_{45}) - \tilde{a}_{13} \tilde{a}_{46} (\tilde{a}_{42} + \tilde{a}_{45}) \right] \right. \\ & + \tilde{a}_{45} q^2 \left[ -\tilde{a}_{12} \tilde{a}_{43} (\tilde{a}_{42} + \tilde{a}_{45}) + \tilde{a}_{13} \tilde{a}_{42} (\tilde{a}_{43} + \tilde{a}_{45} - \tilde{a}_{46}) + \tilde{a}_{13} \tilde{a}_{43} \tilde{a}_{46} \right] \\ & \left. + \tilde{a}_{42} \tilde{a}_{45} m_B^2 (\tilde{a}_{12} \tilde{a}_{43} + \tilde{a}_{13} \tilde{a}_{46}) \right) , \end{aligned}$$

$$A_1^{(0,\phi)}(s, q^2) = -6m_B (\tilde{a}_{12} \tilde{a}_{43} + \tilde{a}_{46} (\tilde{a}_{13} - 2(\tilde{a}_{43} + \tilde{a}_{45}))) - 2\tilde{a}_{42} (\tilde{a}_{43} + 2\tilde{a}_{45}) ,$$

$$A_2^{(0,\phi)}(s, q^2) = 0 ,$$

$$\begin{aligned} A_0^{(1,\Phi)}(s, q^2) = & 8 \left( (\tilde{a}_{12} - \tilde{a}_{13}) \left[ s (\tilde{a}_{42} (\tilde{a}_{45} + \tilde{a}_{46}) + 2\tilde{a}_{45} \tilde{a}_{46}) - \tilde{a}_{45} q^2 (2\tilde{a}_{42} + \tilde{a}_{45} + \tilde{a}_{46}) \right] \right. \\ & \left. + \tilde{a}_{45} m_B^2 (\tilde{a}_{12} (2\tilde{a}_{42} + \tilde{a}_{46}) + \tilde{a}_{13} (\tilde{a}_{42} + 2\tilde{a}_{46})) \right) , \end{aligned}$$

$$A_1^{(1,\Phi)}(s, q^2) = -4(\tilde{a}_{12} - \tilde{a}_{13} - 3\tilde{a}_{42} - 4\tilde{a}_{45} - 3\tilde{a}_{46}) ,$$

$$A_2^{(1,\Phi)}(s, q^2) = 0 ,$$

$$\begin{aligned} A_0^{(2,\Phi)}(s, q^2) = & 8 \left( s \left[ \tilde{a}_{12} \tilde{a}_{42} (\tilde{a}_{45} + 3\tilde{a}_{46}) + \tilde{a}_{12} \tilde{a}_{43} (\tilde{a}_{46} - \tilde{a}_{45}) - 4\tilde{a}_{13} \tilde{a}_{42} \tilde{a}_{46} \right] + q^2 \left[ -2\tilde{a}_{12} \tilde{a}_{43} (\tilde{a}_{45} + \tilde{a}_{46}) \right. \right. \\ & \left. \left. + \tilde{a}_{13} \tilde{a}_{42} (\tilde{a}_{45} - \tilde{a}_{46}) + \tilde{a}_{13} \tilde{a}_{43} (\tilde{a}_{45} + 3\tilde{a}_{46}) \right] + m_B^2 (\tilde{a}_{12} \tilde{a}_{43} (\tilde{a}_{45} + 2\tilde{a}_{46}) + \tilde{a}_{13} \tilde{a}_{42} \tilde{a}_{46}) \right) , \end{aligned}$$

$$A_1^{(2,\Phi)}(s, q^2) = -4(2\tilde{a}_{13} - 3\tilde{a}_{42} - 3\tilde{a}_{43} - 2\tilde{a}_{45} - 6\tilde{a}_{46}) ,$$

$$A_2^{(2,\Phi)}(s, q^2) = 0 ,$$

$$A_0^{(3,\Phi)}(s, q^2) = 24 \left( (\tilde{a}_{12} - \tilde{a}_{13})(\tilde{a}_{42} + \tilde{a}_{45})(\tilde{a}_{42}s - \tilde{a}_{43}q^2) + \tilde{a}_{42}m_B^2(\tilde{a}_{12}\tilde{a}_{43} + \tilde{a}_{13}\tilde{a}_{45}) \right),$$

$$A_1^{(3,\Phi)}(s, q^2) = 12 (\tilde{a}_{12} - \tilde{a}_{13} + 2(\tilde{a}_{42} + \tilde{a}_{43} + \tilde{a}_{45})),$$

$$A_2^{(3,\Phi)}(s, q^2) = 0,$$

$$\begin{aligned} A_0^{(4,\Phi)}(s, q^2) = & -8 \left( \tilde{a}_{45} \left[ m_B^2 q^2 (\tilde{a}_{12}\tilde{a}_{43}(\tilde{a}_{42}(\tilde{a}_{43} - 4\tilde{a}_{42}) - \tilde{a}_{45}(2\tilde{a}_{42} + \tilde{a}_{43})) + \tilde{a}_{13}(\tilde{a}_{42}^2(2\tilde{a}_{43} + \tilde{a}_{45} - 2\tilde{a}_{46}) \right. \right. \\ & + \tilde{a}_{42}\tilde{a}_{43}(\tilde{a}_{43} + 2\tilde{a}_{45}) + 2\tilde{a}_{43}^2\tilde{a}_{46})) + q^4(\tilde{a}_{42} - \tilde{a}_{43})(2\tilde{a}_{12}\tilde{a}_{43}(\tilde{a}_{42} + \tilde{a}_{45}) - \tilde{a}_{13}(\tilde{a}_{42}(2\tilde{a}_{43} \\ & + \tilde{a}_{45} - \tilde{a}_{46}) + \tilde{a}_{43}(\tilde{a}_{45} + \tilde{a}_{46}))) + \tilde{a}_{42}m_B^4(\tilde{a}_{12}\tilde{a}_{43}(2\tilde{a}_{42} + \tilde{a}_{43}) + \tilde{a}_{13}\tilde{a}_{46}(\tilde{a}_{42} + 2\tilde{a}_{43})) \Big] \\ & + s \left[ \tilde{a}_{42}m_B^2(\tilde{a}_{12}\tilde{a}_{46}(\tilde{a}_{42}(2\tilde{a}_{43} + \tilde{a}_{45}) + \tilde{a}_{43}(\tilde{a}_{43} + 2\tilde{a}_{45})) + 2\tilde{a}_{12}\tilde{a}_{45}(\tilde{a}_{42} - \tilde{a}_{43})(\tilde{a}_{42} + \tilde{a}_{43}) \right. \\ & - \tilde{a}_{13}\tilde{a}_{46}(\tilde{a}_{42}^2 + 2\tilde{a}_{42}\tilde{a}_{43} - \tilde{a}_{42}\tilde{a}_{45} + 4\tilde{a}_{43}\tilde{a}_{45})) - q^2(\tilde{a}_{42} - \tilde{a}_{43})(\tilde{a}_{12}(2\tilde{a}_{42}^2\tilde{a}_{45} + 2\tilde{a}_{42}\tilde{a}_{43}\tilde{a}_{46} \\ & + \tilde{a}_{42}\tilde{a}_{45}(\tilde{a}_{45} + \tilde{a}_{46}) + \tilde{a}_{43}\tilde{a}_{45}(\tilde{a}_{45} + \tilde{a}_{46})) - \tilde{a}_{13}(\tilde{a}_{42}\tilde{a}_{45}(\tilde{a}_{42} + \tilde{a}_{43} + 2\tilde{a}_{45}) \\ & + \tilde{a}_{42}\tilde{a}_{46}(\tilde{a}_{42} + \tilde{a}_{43}) + 2\tilde{a}_{43}\tilde{a}_{45}\tilde{a}_{46})) \Big] + \tilde{a}_{42}s^2(\tilde{a}_{42} - \tilde{a}_{43})(\tilde{a}_{12}\tilde{a}_{46}(\tilde{a}_{42} + \tilde{a}_{43} + 2\tilde{a}_{45}) \\ & + \tilde{a}_{12}\tilde{a}_{45}(\tilde{a}_{42} - \tilde{a}_{43}) - 2\tilde{a}_{13}\tilde{a}_{46}(\tilde{a}_{42} + \tilde{a}_{45}))) \Big), \end{aligned}$$

$$\begin{aligned} A_1^{(4,\Phi)}(s, q^2) = & -4 \left( q^2 \left[ -\tilde{a}_{12}(\tilde{a}_{42}\tilde{a}_{43} + 2\tilde{a}_{43}^2 + 2\tilde{a}_{43}(2\tilde{a}_{45} + \tilde{a}_{46}) + \tilde{a}_{45}(\tilde{a}_{45} + \tilde{a}_{46})) + \tilde{a}_{13}(\tilde{a}_{42}(2\tilde{a}_{43} \right. \right. \\ & + \tilde{a}_{45} - \tilde{a}_{46}) + \tilde{a}_{43}^2 + 2\tilde{a}_{43}(2\tilde{a}_{45} + \tilde{a}_{46}) + \tilde{a}_{45}(\tilde{a}_{45} + \tilde{a}_{46})) - 3\tilde{a}_{42}^2\tilde{a}_{43} - 8\tilde{a}_{42}^2\tilde{a}_{45} \\ & + 3\tilde{a}_{42}\tilde{a}_{43}^2 + 6\tilde{a}_{42}\tilde{a}_{43}\tilde{a}_{45} - 2\tilde{a}_{42}\tilde{a}_{45}^2 + 2\tilde{a}_{43}^2\tilde{a}_{46} + 2\tilde{a}_{43}\tilde{a}_{45}^2 \Big] + s \left[ \tilde{a}_{12}(3\tilde{a}_{42}^2 + \tilde{a}_{42}(-\tilde{a}_{43} \right. \\ & + 5\tilde{a}_{45} + 3\tilde{a}_{46}) + \tilde{a}_{43}^2 - 2\tilde{a}_{43}\tilde{a}_{45} + 2\tilde{a}_{45}\tilde{a}_{46}) + 2\tilde{a}_{46}(\tilde{a}_{13}(-2\tilde{a}_{42} + \tilde{a}_{43} - \tilde{a}_{45}) \\ & + \tilde{a}_{42}^2 + \tilde{a}_{42}\tilde{a}_{45} - \tilde{a}_{43}(2\tilde{a}_{43} + \tilde{a}_{45})) - \tilde{a}_{42}(2\tilde{a}_{45}(2\tilde{a}_{13} - 2\tilde{a}_{42} + \tilde{a}_{43}) + 3\tilde{a}_{13}\tilde{a}_{42} \\ & + 3\tilde{a}_{43}(\tilde{a}_{43} - \tilde{a}_{42})) \Big] + 2\tilde{a}_{45}(\tilde{a}_{42}(3\tilde{a}_{12} + \tilde{a}_{13} - \tilde{a}_{42}) - 2\tilde{a}_{43}(\tilde{a}_{12} - 2\tilde{a}_{42}) + \tilde{a}_{43}^2) \\ & + m_B^2(\tilde{a}_{12}\tilde{a}_{43}(\tilde{a}_{42} - \tilde{a}_{43} + 2\tilde{a}_{45}) + \tilde{a}_{12}\tilde{a}_{46}(2\tilde{a}_{43} + \tilde{a}_{45}) + \tilde{a}_{13}\tilde{a}_{46}(\tilde{a}_{42} - 2\tilde{a}_{43} + 2\tilde{a}_{45}) \\ & + 2\tilde{a}_{42}\tilde{a}_{45}(2\tilde{a}_{13} + 4\tilde{a}_{42} + \tilde{a}_{43}) + 3\tilde{a}_{42}\tilde{a}_{43}(\tilde{a}_{42} + \tilde{a}_{43}) + 2\tilde{a}_{43}\tilde{a}_{46}(2\tilde{a}_{43} + \tilde{a}_{45}) \Big] \\ & + 2\tilde{a}_{46}(\tilde{a}_{42}(\tilde{a}_{12} - 3\tilde{a}_{13} + 4\tilde{a}_{43}) + 4\tilde{a}_{45}(\tilde{a}_{42} + \tilde{a}_{43}))) \Big), \end{aligned}$$



$$A_2^{(4,\Phi)}(s, q^2) = 4(2\tilde{a}_{13} - 3\tilde{a}_{42} - 4(\tilde{a}_{43} + \tilde{a}_{45}) - 3\tilde{a}_{46}),$$

$$\begin{aligned} A_0^{(5,\Phi)}(s, q^2) = & -8 \left( s \left[ \tilde{a}_{42} m_B^2 (\tilde{a}_{12} \tilde{a}_{45} (2\tilde{a}_{42}^2 + \tilde{a}_{42}(\tilde{a}_{45} - \tilde{a}_{43}) - 2\tilde{a}_{43} \tilde{a}_{45}) + \tilde{a}_{12} \tilde{a}_{46} (\tilde{a}_{42} (2\tilde{a}_{43} + \tilde{a}_{45}) \right. \right. \\ & + \tilde{a}_{45} (\tilde{a}_{43} + 2\tilde{a}_{45})) - \tilde{a}_{13} \tilde{a}_{46} (\tilde{a}_{42}^2 + \tilde{a}_{42} \tilde{a}_{45} + 4\tilde{a}_{45}^2) \Big) - q^2 (\tilde{a}_{42} - \tilde{a}_{45}) (\tilde{a}_{12} (2\tilde{a}_{42}^2 \tilde{a}_{45} \\ & + 2\tilde{a}_{42} \tilde{a}_{43} \tilde{a}_{46} + \tilde{a}_{42} \tilde{a}_{45} (\tilde{a}_{45} + \tilde{a}_{46}) + \tilde{a}_{43} \tilde{a}_{45} (\tilde{a}_{45} + \tilde{a}_{46})) - \tilde{a}_{13} (\tilde{a}_{42} \tilde{a}_{45} (\tilde{a}_{42} + \tilde{a}_{43} \\ & + 2\tilde{a}_{45}) + \tilde{a}_{42} \tilde{a}_{46} (\tilde{a}_{42} + \tilde{a}_{43}) + 2\tilde{a}_{43} \tilde{a}_{45} \tilde{a}_{46})) \Big] + \tilde{a}_{45} \left[ m_B^2 q^2 (\tilde{a}_{13} (\tilde{a}_{42}^2 (2\tilde{a}_{43} + \tilde{a}_{45} \right. \\ & - 2\tilde{a}_{46}) + \tilde{a}_{42} \tilde{a}_{46} (\tilde{a}_{43} - \tilde{a}_{45}) + \tilde{a}_{42} \tilde{a}_{45} (\tilde{a}_{43} + 2\tilde{a}_{45}) + 2\tilde{a}_{43} \tilde{a}_{45} \tilde{a}_{46}) - \tilde{a}_{12} \tilde{a}_{43} (4\tilde{a}_{42}^2 \\ & + \tilde{a}_{42} \tilde{a}_{45} + \tilde{a}_{45}^2) \Big) - q^4 (\tilde{a}_{42} - \tilde{a}_{45}) (-2\tilde{a}_{12} \tilde{a}_{43} (\tilde{a}_{42} + \tilde{a}_{45}) + \tilde{a}_{13} \tilde{a}_{42} (2\tilde{a}_{43} + \tilde{a}_{45} \\ & - \tilde{a}_{46}) + \tilde{a}_{13} \tilde{a}_{43} (\tilde{a}_{45} + \tilde{a}_{46})) + \tilde{a}_{42} m_B^4 (\tilde{a}_{12} \tilde{a}_{43} (2\tilde{a}_{42} + \tilde{a}_{45}) + \tilde{a}_{13} \tilde{a}_{46} (\tilde{a}_{42} + 2\tilde{a}_{45})) \Big] \\ & \left. + \tilde{a}_{42} s^2 (\tilde{a}_{42} - \tilde{a}_{45}) (\tilde{a}_{12} \tilde{a}_{46} (\tilde{a}_{42} + \tilde{a}_{43} + 2\tilde{a}_{45}) + \tilde{a}_{12} \tilde{a}_{45} (\tilde{a}_{42} - \tilde{a}_{43}) - 2\tilde{a}_{13} \tilde{a}_{46} (\tilde{a}_{42} + \tilde{a}_{45})) \right) \Big), \end{aligned}$$

$$\begin{aligned} A_1^{(5,\Phi)}(s, q^2) = & -4 \left( s \left[ \tilde{a}_{12} (3\tilde{a}_{42}^2 + \tilde{a}_{46} (3\tilde{a}_{42} + \tilde{a}_{43} + \tilde{a}_{45}) - \tilde{a}_{42} \tilde{a}_{43} + 5\tilde{a}_{42} \tilde{a}_{45} - \tilde{a}_{43} \tilde{a}_{45}) \right. \right. \\ & + 2\tilde{a}_{46} (-2\tilde{a}_{13} \tilde{a}_{42} + \tilde{a}_{42}^2 + \tilde{a}_{42} \tilde{a}_{43} - \tilde{a}_{45} (\tilde{a}_{43} + 2\tilde{a}_{45})) - \tilde{a}_{42} (\tilde{a}_{45} (4\tilde{a}_{13} - 4\tilde{a}_{42} + \tilde{a}_{43}) \\ & + 3\tilde{a}_{42} (\tilde{a}_{13} - \tilde{a}_{43}) + 4\tilde{a}_{45}^2) \Big] + q^2 [-\tilde{a}_{12} (\tilde{a}_{42} \tilde{a}_{43} + 2\tilde{a}_{43} (3\tilde{a}_{45} + \tilde{a}_{46}) + \tilde{a}_{45} (\tilde{a}_{45} + \tilde{a}_{46})) \\ & + \tilde{a}_{13} (\tilde{a}_{42} (2\tilde{a}_{43} + \tilde{a}_{45} - \tilde{a}_{46}) + 5\tilde{a}_{43} \tilde{a}_{45} + 3\tilde{a}_{43} \tilde{a}_{46} + \tilde{a}_{45}^2) - 3\tilde{a}_{42}^2 \tilde{a}_{43} - 8\tilde{a}_{42}^2 \tilde{a}_{45} \\ & + \tilde{a}_{42} \tilde{a}_{43} \tilde{a}_{45} + 6\tilde{a}_{42} \tilde{a}_{45}^2 + 2\tilde{a}_{45}^3 + 2\tilde{a}_{45}^2 \tilde{a}_{46}] + m_B^2 [\tilde{a}_{12} \tilde{a}_{43} (\tilde{a}_{42} + \tilde{a}_{45}) + \tilde{a}_{12} \tilde{a}_{46} (2\tilde{a}_{43} \\ & + \tilde{a}_{45}) + \tilde{a}_{42} \tilde{a}_{45} (4\tilde{a}_{13} + \tilde{a}_{43} + 4\tilde{a}_{45}) + \tilde{a}_{13} \tilde{a}_{42} \tilde{a}_{46} + \tilde{a}_{42}^2 (3\tilde{a}_{43} + 8\tilde{a}_{45}) \\ & + 2\tilde{a}_{45} \tilde{a}_{46} (\tilde{a}_{43} + 2\tilde{a}_{45})] + 2\tilde{a}_{46} (\tilde{a}_{42} (\tilde{a}_{12} - 3\tilde{a}_{13} + 4\tilde{a}_{43}) + 4\tilde{a}_{45} (\tilde{a}_{42} + \tilde{a}_{43})) \\ & \left. + 2\tilde{a}_{45} (\tilde{a}_{12} (3\tilde{a}_{42} - 2\tilde{a}_{43}) + \tilde{a}_{42} (\tilde{a}_{13} - \tilde{a}_{42} + 3\tilde{a}_{43}) + \tilde{a}_{45} (\tilde{a}_{42} + \tilde{a}_{43})) \right) \Big), \end{aligned}$$

$$A_2^{(5,\Phi)}(s, q^2) = 4(2\tilde{a}_{13} - 3\tilde{a}_{42} - 3\tilde{a}_{43} - 5\tilde{a}_{45} - 3\tilde{a}_{46}),$$

$$\begin{aligned} A_0^{(6,\Phi)}(s, q^2) = & -8 \left( s \left\{ q^2 (\tilde{a}_{45} - \tilde{a}_{46}) [\tilde{a}_{12} \tilde{a}_{45} (2\tilde{a}_{42}^2 + \tilde{a}_{45} (\tilde{a}_{42} + \tilde{a}_{43})) + \tilde{a}_{12} \tilde{a}_{46} (\tilde{a}_{45} (\tilde{a}_{42} + \tilde{a}_{43}) + 2\tilde{a}_{42} \tilde{a}_{43}) \right. \right. \\ & \left. \left. - \tilde{a}_{13} \tilde{a}_{46} (\tilde{a}_{42} (\tilde{a}_{42} + \tilde{a}_{43}) + 2\tilde{a}_{43} \tilde{a}_{45}) - \tilde{a}_{13} \tilde{a}_{42} \tilde{a}_{45} (\tilde{a}_{42} + \tilde{a}_{43} + 2\tilde{a}_{45}) \right] \right. \end{aligned}$$

$$\begin{aligned}
& + \tilde{a}_{42} m_B^2 \left[ \tilde{a}_{46}^2 (\tilde{a}_{45} (\tilde{a}_{12} + \tilde{a}_{13}) + 2\tilde{a}_{12}\tilde{a}_{43} - \tilde{a}_{13}\tilde{a}_{42}) + 2\tilde{a}_{45}\tilde{a}_{46} (\tilde{a}_{12} (\tilde{a}_{42} + \tilde{a}_{45}) \right. \\
& \left. - \tilde{a}_{13} (\tilde{a}_{42} + 2\tilde{a}_{45})) + \tilde{a}_{12}\tilde{a}_{45}^2 (\tilde{a}_{42} - 2\tilde{a}_{43}) \right] \Big\} + \tilde{a}_{45} \left[ m_B^2 q^2 (\tilde{a}_{12}\tilde{a}_{43} (\tilde{a}_{45} (\tilde{a}_{42} - \tilde{a}_{45}) \right. \\
& \left. - 2\tilde{a}_{46} (2\tilde{a}_{42} + \tilde{a}_{45})) + \tilde{a}_{13} (2\tilde{a}_{43}\tilde{a}_{46} (\tilde{a}_{42} + \tilde{a}_{45}) + \tilde{a}_{42}\tilde{a}_{45} (\tilde{a}_{43} + 2\tilde{a}_{45}) + \tilde{a}_{46}^2 (\tilde{a}_{43} - 2\tilde{a}_{42})) \right) \\
& + q^4 (\tilde{a}_{45} - \tilde{a}_{46}) (-2\tilde{a}_{12}\tilde{a}_{43} (\tilde{a}_{42} + \tilde{a}_{45}) + \tilde{a}_{13}\tilde{a}_{42} (2\tilde{a}_{43} + \tilde{a}_{45} - \tilde{a}_{46}) + \tilde{a}_{13}\tilde{a}_{43} (\tilde{a}_{45} + \tilde{a}_{46})) \\
& + \tilde{a}_{42} m_B^4 (\tilde{a}_{12}\tilde{a}_{43} (\tilde{a}_{45} + 2\tilde{a}_{46}) + \tilde{a}_{13}\tilde{a}_{46} (2\tilde{a}_{45} + \tilde{a}_{46})) \Big] - \tilde{a}_{42} s^2 (\tilde{a}_{45} - \tilde{a}_{46}) (\tilde{a}_{12}\tilde{a}_{46} (\tilde{a}_{42} \\
& + \tilde{a}_{43} + 2\tilde{a}_{45}) + \tilde{a}_{12}\tilde{a}_{45} (\tilde{a}_{42} - \tilde{a}_{43}) - 2\tilde{a}_{13}\tilde{a}_{46} (\tilde{a}_{42} + \tilde{a}_{45})) \Big),
\end{aligned}$$

$$\begin{aligned}
A_1^{(6,\Phi)}(s, q^2) = & -4 \Big( s \left[ \tilde{a}_{12} (3\tilde{a}_{42}^2 + \tilde{a}_{42} (5\tilde{a}_{45} + 2\tilde{a}_{46}) - \tilde{a}_{43}\tilde{a}_{45} + \tilde{a}_{46} (\tilde{a}_{45} + \tilde{a}_{46})) + 2\tilde{a}_{46}^2 (-\tilde{a}_{13} + \tilde{a}_{42} \right. \\
& + 2(\tilde{a}_{43} + \tilde{a}_{45})) + \tilde{a}_{46} (-2\tilde{a}_{13}\tilde{a}_{42} + \tilde{a}_{42}\tilde{a}_{43} - 2\tilde{a}_{45} (\tilde{a}_{43} + 2\tilde{a}_{45})) - \tilde{a}_{42} (\tilde{a}_{13} (3\tilde{a}_{42} + 4\tilde{a}_{45}) \\
& + \tilde{a}_{45} (\tilde{a}_{43} + 4\tilde{a}_{45})) \Big] + q^2 \left[ -\tilde{a}_{12} (3\tilde{a}_{42}\tilde{a}_{43} + \tilde{a}_{45} (6\tilde{a}_{43} + \tilde{a}_{45} + \tilde{a}_{46})) + \tilde{a}_{13} (\tilde{a}_{42} (3\tilde{a}_{43} \right. \\
& + \tilde{a}_{45} - 2\tilde{a}_{46}) + 5\tilde{a}_{43}\tilde{a}_{45} + 2\tilde{a}_{43}\tilde{a}_{46} + \tilde{a}_{45}^2 + \tilde{a}_{46}^2) - \tilde{a}_{42}\tilde{a}_{46} (\tilde{a}_{43} + 6\tilde{a}_{45}) + \tilde{a}_{42}\tilde{a}_{45} (\tilde{a}_{43} \\
& + 8\tilde{a}_{45}) - 2\tilde{a}_{46}^2 (\tilde{a}_{43} + \tilde{a}_{45}) + 2\tilde{a}_{45}^3 \Big] + m_B^2 \left[ \tilde{a}_{12} (3\tilde{a}_{42}\tilde{a}_{43} + \tilde{a}_{45} (\tilde{a}_{43} + \tilde{a}_{46})) \right. \\
& + \tilde{a}_{46} (2\tilde{a}_{13}\tilde{a}_{42} + \tilde{a}_{42} (\tilde{a}_{43} + 6\tilde{a}_{45}) + 2\tilde{a}_{45} (\tilde{a}_{43} + 2\tilde{a}_{45})) + \tilde{a}_{42}\tilde{a}_{45} (4\tilde{a}_{13} + \tilde{a}_{43} + 4\tilde{a}_{45}) \\
& + \tilde{a}_{46}^2 (2(\tilde{a}_{43} + \tilde{a}_{45}) - \tilde{a}_{13}) \Big] + 2\tilde{a}_{46} (\tilde{a}_{42} (\tilde{a}_{12} - 3\tilde{a}_{13} + 4\tilde{a}_{43}) + 3\tilde{a}_{45} (\tilde{a}_{42} + \tilde{a}_{43})) \\
& \left. + 2\tilde{a}_{45} (3\tilde{a}_{12}\tilde{a}_{42} - 2\tilde{a}_{12}\tilde{a}_{43} + \tilde{a}_{13}\tilde{a}_{42} + \tilde{a}_{45} (\tilde{a}_{42} + \tilde{a}_{43}) + 4\tilde{a}_{42}\tilde{a}_{43}) \right) \Big),
\end{aligned}$$

$$A_2^{(6,\Phi)}(s, q^2) = 4(2\tilde{a}_{13} - 4\tilde{a}_{42} - 3\tilde{a}_{43} - 5\tilde{a}_{45} - 2\tilde{a}_{46}).$$

$$\bullet \underline{C_i^{(j,\phi/\Phi)}}:$$

The coefficients used in the  $I^{(C^4)}$  function ( $C$ ) are given below:

$$\begin{aligned}
C_0^{(0,\phi)}(s, q^2) = & -4 m_B (\hat{\omega} - 1) \Big( (\hat{\omega} - 1) \left[ q^2 (3x_2^2 x_3 - 3x_2^2 + 3x_2 x_3^2 - 2x_2 \hat{\omega} (x_2 + x_3 - 1)^2 - 3x_2 x_3 \right. \\
& + 3x_2 - x_3^2 + x_3) + m_B^2 (2\hat{\omega}^2 (x_2 + x_3 - 1)^2 (x_2 + x_3) - \hat{\omega} (x_2 + x_3 - 1) (x_2 (5x_3 \\
& - 3) + x_3 (5x_3 - 2)) + (x_3 - 1) x_3 (3x_2 + 3x_3 + 1) \Big] + s (2x_2 \hat{\omega}^2 (x_2 + x_3 - 1)^2 \\
& - \hat{\omega} (x_2 + x_3 - 1) (x_2 (5x_3 - 3) + x_3) + (3x_2 + 1) (x_3 - 1) x_3) \Big),
\end{aligned}$$

$$C_1^{(0,\phi)}(s, q^2) = -2m_B(\hat{\omega} - 1)(2(3x_2 - 5)\hat{\omega} + x_3(6\hat{\omega} - 9) + 6),$$

$$C_2^{(0,\phi)}(s, q^2) = 0,$$

$$\begin{aligned} C_0^{(1,\phi)}(s, q^2) = & 8\left((\hat{\omega} - 1)[x_2 q^2(x_2^2 - 4\hat{\omega}(x_2 + x_3 - 1)^2 + 5x_2x_3 - 5x_2 + 4x_3^2 - 6x_3 + 4) \right. \\ & + m_B^2(x_3(x_2^2 + 5(x_2 - 1)x_3 - 4x_2 + 4x_3^2 + 1) - \hat{\omega}(x_2 + x_3 - 1)((9x_2 - 5)x_3 \\ & + (x_2 - 4)x_2 + 8x_3^2) + 4\hat{\omega}^2(x_2 + x_3 - 1)^2(x_2 + x_3))] + x_2 s (\hat{\omega}(x_2 + x_3 - 1) \\ & \left. - x_3)(4\hat{\omega}(x_2 + x_3 - 1) - x_2 - 4x_3 + 4)\right), \end{aligned}$$

$$C_1^{(1,\phi)}(s, q^2) = 4(2\hat{\omega}(6x_2 + 6x_3 - 7) - 3x_2 - 12x_3 + 8),$$

$$C_2^{(1,\phi)}(s, q^2) = 0,$$

$$\begin{aligned} C_0^{(2,\phi)}(s, q^2) = & -8\left((\hat{\omega} - 1)[m_B^2(x_2^2\hat{\omega} + 2x_2(x_3 - 1)(2\hat{\omega} - 1) + 3(x_3 - 1)x_3(\hat{\omega} - 1)) \right. \\ & \left. - x_2q^2(x_2 + 2x_3 - 2)] + x_2 s ((x_2 - 2)\hat{\omega} + 2x_3(\hat{\omega} - 1) + 2)\right), \end{aligned}$$

$$C_1^{(2,\phi)}(s, q^2) = -12,$$

$$C_2^{(2,\phi)}(s, q^2) = 0,$$

$$\begin{aligned} C_0^{(3,\phi)}(s, q^2) = & 8\left((\hat{\omega} - 1)[m_B^2(\hat{\omega}(-8x_2x_3 - 3(x_2 - 1)x_2 - 5x_3^2 + 2x_3) + 2\hat{\omega}^2(x_2 + x_3 - 1)(x_2 + x_3), \right. \\ & + x_3(3x_2 + 3x_3 + 1)) - q^2(x_2(2\hat{\omega} - 3)(x_2 + x_3 - 1) + x_3)] \\ & \left. + s(x_3(\hat{\omega} - 1)(2x_2\hat{\omega} - 3x_2 - 1) + (x_2 - 1)x_2\hat{\omega}(2\hat{\omega} - 3))\right), \end{aligned}$$

$$C_1^{(3,\phi)}(s, q^2) = 8(2\hat{\omega} - 3),$$

$$C_2^{(3,\phi)}(s, q^2) = 0,$$

$$\begin{aligned} C_0^{(4,\phi)}(s, q^2) = & 8\left((\hat{\omega} - 1)s\left[x_2 q^2(4\hat{\omega}(x_2 + x_3 - 1)^2 - 5x_2x_3 + 4x_2 - 4x_3^2 + 6x_3 - 4) \right. \right. \\ & + m_B^2(-\hat{\omega}^2(x_2 + x_3 - 1)(6x_2^2 + 5x_2(3x_3 - 2) + x_3(4x_3 - 3)) \\ & \left. \left. + \hat{\omega}(2x_2^2(7x_3 - 4) + x_2(5x_3 - 4)(5x_3 - 2) + (x_3 - 1)x_3(8x_3 - 3))\right) \right. \end{aligned}$$

$$\begin{aligned}
& + 2x_2\hat{\omega}^3(x_2 + x_3 - 1)^2 - 4(x_3 - 1)x_3(2x_2 + x_3)) \Big] \\
& + (\hat{\omega} - 1)^2 \Big[ m_B^2 q^2 ( - 2x_2^3(\hat{\omega} - 2)\hat{\omega} + x_2^2 ( - 4(x_3 - 1)\hat{\omega}^2 + (11x_3 - 10)\hat{\omega} \\
& - 5x_3 + 4) - x_2(\hat{\omega} - 1) ( - 5x_3^2 + 2(x_3 - 1)^2\hat{\omega} + 6x_3 - 4) + x_3(x_3(-\hat{\omega}) \\
& + x_3 + \hat{\omega} - 1)) - x_2^2 q^4 (x_2 + x_3 - 1) + m_B^4 (\hat{\omega} (x_2^2(7x_3 - 4) + x_2(x_3(17x_3 \\
& - 18) + 4) + (x_3 - 1)x_3(10x_3 - 3)) - \hat{\omega}^2(x_2 + x_3 - 1)((11x_2 - 5)x_3 \\
& + 3(x_2 - 2)x_2 + 8x_3^2) + 2\hat{\omega}^3(x_2 + x_3 - 1)^2(x_2 + x_3) - 4(x_3 - 1)x_3(x_2 + x_3)) \Big] \\
& - x_2 s^2 (3x_2\hat{\omega} + 4x_3(\hat{\omega} - 1) - 4\hat{\omega} + 4) (\hat{\omega}(x_2 + x_3 - 1) - x_3) \Big),
\end{aligned}$$

$$\begin{aligned}
C_1^{(4,\phi)}(s, q^2) = & 4 \Big( (\hat{\omega} - 1) [q^2 (\hat{\omega}(x_2 + x_3 - 1) + x_2 - x_3 + 2) + m_B^2 (\hat{\omega}(6x_2\hat{\omega} - 8x_2 - 10\hat{\omega} + 17) \\
& + x_3(\hat{\omega} - 1)(6\hat{\omega} - 11) - 8) + 2 (-2\hat{\omega}(x_2 + x_3 - 1) + x_2 + 2x_3 - 1)] \\
& - s (\hat{\omega} ((x_2 - 1)\hat{\omega} + 8x_2 - 13) + x_3(\hat{\omega} - 1)(\hat{\omega} + 11) + 8) \Big),
\end{aligned}$$

$$C_2^{(4,\phi)}(s, q^2) = 0,$$

$$\begin{aligned}
C_0^{(5,\phi)}(s, q^2) = & -8 \Big( (\hat{\omega} - 1) s \Big[ (x_2 - 1)x_2 q^2 (4\hat{\omega}(x_2 + x_3 - 1)^2 - 5x_2x_3 + 4x_2 - 4x_3^2 + 6x_3 - 4) \\
& + m_B^2 (\hat{\omega}(x_2 + x_3 - 1) - x_3) \Big( -\hat{\omega} (3(3x_2 - 1)x_3^2 + 3(x_2(5x_2 - 7) + 1)x_3 \\
& + 2(x_2 - 1)x_2(3x_2 - 5)) + 2x_2\hat{\omega}^2(x_2 + x_3 - 1)^2 + (x_3 - 1)((7x_2 - 3)x_3 \\
& + 8(x_2 - 1)x_2) \Big) \Big] + (\hat{\omega} - 1)^2(x_2 + x_3 - 1) \Big[ m_B^2 q^2 ( - 2x_2^3(\hat{\omega} - 2)\hat{\omega} \\
& + x_2^2 ( - 4(x_3 - 1)\hat{\omega}^2 + (9x_3 - 10)\hat{\omega} - 5x_3 + 4) - x_2(\hat{\omega} - 1) ( - 3x_3^2 \\
& + 2(x_3 - 1)^2\hat{\omega} + 5x_3 - 4) + x_3(x_3(-\hat{\omega}) + x_3 + \hat{\omega} - 1)) - (x_2 - 1)x_2^2 q^4 \\
& + m_B^4 (\hat{\omega}(x_2 + x_3 - 1) - x_3) (x_2^2\hat{\omega}(2\hat{\omega} - 3) + 2x_2(\hat{\omega} - 1)(2x_3(\hat{\omega} - 1) - \hat{\omega} + 2) \\
& + (x_3 - 1)x_3(\hat{\omega} - 1)(2\hat{\omega} - 3)) \Big] - (x_2 - 1)x_2 s^2 (3x_2\hat{\omega} + 4x_3(\hat{\omega} - 1) - 4\hat{\omega} \\
& + 4) (\hat{\omega}(x_2 + x_3 - 1) - x_3) \Big),
\end{aligned}$$

$$C_1^{(5,\phi)}(s, q^2) = -4 \left( s \left( -\hat{\omega} (13x_2^2 + x_2(20x_3 - 29) + x_3(4x_3 - 17) + 17) + \hat{\omega}^2(x_2 + x_3 - 1) \right. \right.$$

$$\left. (2x_2 + 2x_3 - 1) + 2(x_2(8x_3 - 5) + (x_3 - 7)x_3 + 5) \right) - (\hat{\omega} - 1)q^2 \left( -5x_2^2 \right.$$

$$+ \hat{\omega}(x_2 + x_3)(2x_2 + 2x_3 - 3) - 4x_2x_3 + 4x_2 - 2x_3^2 + \hat{\omega} + 4) + m_B^2(\hat{\omega} - 1)$$

$$\left( -\hat{\omega} (13x_2^2 + x_2(36x_3 - 33) + x_3(23x_3 - 38) + 17) + 2\hat{\omega}^2(x_2 + x_3 - 1)(5x_2 + 5x_3 - 6) \right.$$

$$+ 16x_2x_3 - 10x_2 + 13x_3^2 - 19x_3 + 10) + 2\hat{\omega} (4x_2^2 + x_2(12x_3 - 13) + 8(x_3 - 2)x_3)$$

$$\left. - 4\hat{\omega}^2(x_2 + x_3 - 1)(2x_2 + 2x_3 - 3) + 2(4x_2 + 6x_3 + 7\hat{\omega} - 1) - 2(x_2 + 2x_3)^2 \right),$$

$$C_2^{(5,\phi)}(s, q^2) = -4(2\hat{\omega} - 3),$$

$$C_0^{(6,\phi)}(s, q^2) = 8 \left( (\hat{\omega} - 1) s \left[ x_2^2 q^2 (4\hat{\omega}(x_2 + x_3 - 1)^2 - 5x_2x_3 + 4x_2 - 4x_3^2 + 6x_3 - 4) \right. \right.$$

$$+ m_B^2 (\hat{\omega} (2x_2^3(7x_3 - 4) + x_2^2(30x_3^2 - 38x_3 + 11) + x_2(x_3 - 1)(x_3(16x_3 - 13) + 3)$$

$$+ 2(x_3 - 1)^2x_3) - \hat{\omega}^2(x_2 + x_3 - 1)((11x_2 + 1)x_3^2 + (x_2(17x_2 - 15) - 1)x_3$$

$$+ x_2(6(x_2 - 2)x_2 + 5)) + 2x_2\hat{\omega}^3(x_2 + x_3 - 1)^3 - (x_3 - 1)x_3(x_2(8x_2 + 7x_3$$

$$- 3) + x_3 - 1)) \Big] + (\hat{\omega} - 1)^2(x_2 + x_3 - 1) \left[ m_B^4 (\hat{\omega} (x_2^2(7x_3 - 4) + 3x_2(5(x_3 - 1)x_3 \right.$$

$$+ 1) + x_3^2(8x_3 - 9) + x_3) - \hat{\omega}^2(x_2 + x_3 - 1)(3x_2^2 + 5x_2(2x_3 - 1) + x_3(7x_3 - 4))$$

$$+ 2\hat{\omega}^3(x_2 + x_3 - 1)^2(x_2 + x_3) - (x_3 - 1)x_3(4x_2 + 3x_3 + 1)) - q^2(x_3^2q^2$$

$$+ m_B^2(2x_2^3(\hat{\omega} - 2)\hat{\omega} + x_2^2(\hat{\omega} - 1)(4(x_3 - 1)\hat{\omega} - 5x_3 + 4) + x_2(\hat{\omega} - 1)(2(x_3 - 1)^2\hat{\omega}$$

$$- 3x_3(x_3 - 1) - 3) + (x_3 - 1)x_3(\hat{\omega} - 1))) \Big] - x_2^2s^2(3x_2\hat{\omega} + 4x_3(\hat{\omega} - 1) - 4\hat{\omega} + 4)$$

$$\times (\hat{\omega}(x_2 + x_3 - 1) - x_3) \Big),$$

$$C_1^{(6,\phi)}(s, q^2) = 4 \left( s \left( -\hat{\omega} (13x_2^2 + x_2(20x_3 - 21) + x_3(4x_3 - 7) + 4) + 2\hat{\omega}^2(x_2 + x_3 - 1)^2 \right. \right.$$

$$+ 16x_2x_3 - 10x_2 + 2x_3^2 - 3x_3 + 2) - (\hat{\omega} - 1)q^2 \left( -5x_2^2 + 2\hat{\omega}(x_2 + x_3 - 1)^2 \right.$$

$$\left. - 4x_2x_3 + 3x_2 - 2x_3^2 + x_3 + 2) + m_B^2(\hat{\omega} - 1) \left( -\hat{\omega} (13x_2^2 + 36(x_2 - 1)x_3 \right. \right.$$

$$\begin{aligned}
& -31x_2 + 23x_3^2 + 16) + 2\hat{\omega}^2(x_2 + x_3 - 1)(5x_2 + 5x_3 - 6) + 16x_2x_3 - 10x_2 \\
& + 13x_3^2 - 17x_3 + 8) - 8\hat{\omega}^2(x_2 + x_3 - 1)^2 + 4\hat{\omega}(x_2 + 2x_3 - 2)(2x_2 + 2x_3 - 1) \\
& - 8(x_2 - 1)x_3 - 2(x_2 - 3)x_2 - 8x_3^2),
\end{aligned}$$

$$C_2^{(6,\phi)}(s, q^2) = -4(2\hat{\omega} - 3).$$

## 1.4 Diagram in Fig 1D

This section provides the explicit coefficient functions that enter the invariant amplitudes the invariant amplitudes  $I^{(D1)}$ ,  $I^{(D2)}$ . The superscript denotes which three-particle  $B$ -meson distribution amplitudes these coefficient functions are multiplying. Again,  $\hat{m}_b = \frac{m_b}{m_B}$ ,  $\hat{\omega} = \frac{\omega}{m_B}$ .

•  $F_n^{(X)}$ :

The coefficients used in the  $I^{(D1)}$  function are given below:

$$F_1^{(\Psi_{AV})}(q^2, \omega) = \frac{3}{m_b^2}(1 - \hat{\omega})m_B(2\hat{m}_b - 1), \quad F_2^{(\Psi_{VA})}(q^2, \omega) = 0,$$

$$F_1^{(\Psi_V)}(q^2, \omega) = \frac{6}{m_b^2}(1 - \hat{\omega})m_B(2\hat{m}_b - 1), \quad F_2^{(\Psi_V)}(q^2, \omega) = 0,$$

$$F_1^{(X_A)}(q^2, \omega) = -\frac{2}{m_b^2}(1 - 2\hat{m}_b), \quad F_2^{(X_A)}(q^2, \omega) = -\frac{1}{m_b^2}(1 - 2\hat{m}_b)((1 - \hat{\omega})^2 m_B^2 - q^2),$$

$$F_1^{(W_{YA})}(q^2, \omega) = \frac{-4}{(1 - \hat{\omega})^2 m_B^2}, \quad F_2^{(W_{YA})}(q^2, \omega) = \frac{4((1 - \hat{\omega})^3 m_B^2 + q^2(2\hat{\omega} - 1))}{(1 - \hat{\omega})^2 m_B^2},$$

$$F_1^{(\tilde{X}_A)}(q^2, \omega) = F_1^{(X_A)}(q^2, \omega), \quad F_2^{(\tilde{X}_A)}(q^2, \omega) = F_2^{(X_A)}(q^2, \omega),$$

$$F_1^{(\tilde{Y}_A)}(q^2, \omega) = F_1^{(W_{YA})}(q^2, \omega), \quad F_2^{(\tilde{Y}_A)}(q^2, \omega) = F_2^{(W_{YA})}(q^2, \omega).$$

•  $\tilde{F}_n^{(X)}$ :

The coefficients used in the  $I^{(D2)}$  function are given below:

$$\tilde{F}_1^{(\Psi_{AV})}(q^2, \omega) = \frac{3(2\hat{\omega} - 1)}{(1 - \hat{\omega})m_B}, \quad \tilde{F}_2^{(\Psi_{VA})}(q^2, \omega) = 0,$$

$$\tilde{F}_1^{(\Psi_V)}(q^2, \omega) = \frac{6(2\hat{\omega} - 1)}{(1 - \hat{\omega})m_B}, \quad \tilde{F}_2^{(\Psi_V)}(q^2, \omega) = 0,$$

$$\tilde{F}_1^{(X_A)}(q^2, \omega) = \frac{2(3\hat{\omega} - 2)}{(1 - \hat{\omega})^2 m_B^2}, \quad \tilde{F}_2^{(X_A)}(q^2, \omega) = \frac{(1 - \hat{\omega})^2(1 + 2\hat{\omega})m_B^2 + (2\hat{\omega} - 1)q^2}{(1 - \hat{\omega})^2 m_B^2},$$

$$\tilde{F}_1^{(WY_A)}(q^2, \omega) = \frac{-4}{(1 - \hat{\omega})^2 m_B^2}, \quad \tilde{F}_2^{(WY_A)}(q^2, \omega) = \frac{4((1 - \hat{\omega})^3 m_B^2 + q^2(2\hat{\omega} - 1))}{(1 - \hat{\omega})^2 m_B^2},$$

$$\tilde{F}_1^{(\tilde{X}_A)}(q^2, \omega) = \tilde{F}_1^{(X_A)}(q^2, \omega), \quad \tilde{F}_2^{(\tilde{X}_A)}(q^2, \omega) = \tilde{F}_2^{(X_A)}(q^2, \omega),$$

$$\tilde{F}_1^{(\tilde{Y}_A)}(q^2, \omega) = \tilde{F}_1^{(WY_A)}(q^2, \omega), \quad \tilde{F}_2^{(\tilde{Y}_A)}(q^2, \omega) = \tilde{F}_2^{(WY_A)}(q^2, \omega).$$
